# Supplementary material for: PowerRadio: Manipulate Sensor Measurementvia Power GND Radiation
Source: arXiv:2412.18103 source file (2024-12-24)
Supplement: Supplementary file 1 [file Appendix_complete_version.tex]

%% !TEX root = ../main.tex

% \newpage
% \appendix
% \titlespacing*{\section}{0pt}{1ex}{1ex} % 设置 section 标题的间距：左边距，上方距离，下方距离
\section{Appendix}\label{sec: appendix}

\subsection{\textsc{Supplementary Materials of Evaluation}}\label{sec: supplement_eval}
\noindent \textit{(a) Illustration of the experimental setup for a cross-socket attack against a commercial motion detector.}
\begin{figure}[h]
	\centering
	\includegraphics[width=1\linewidth]{./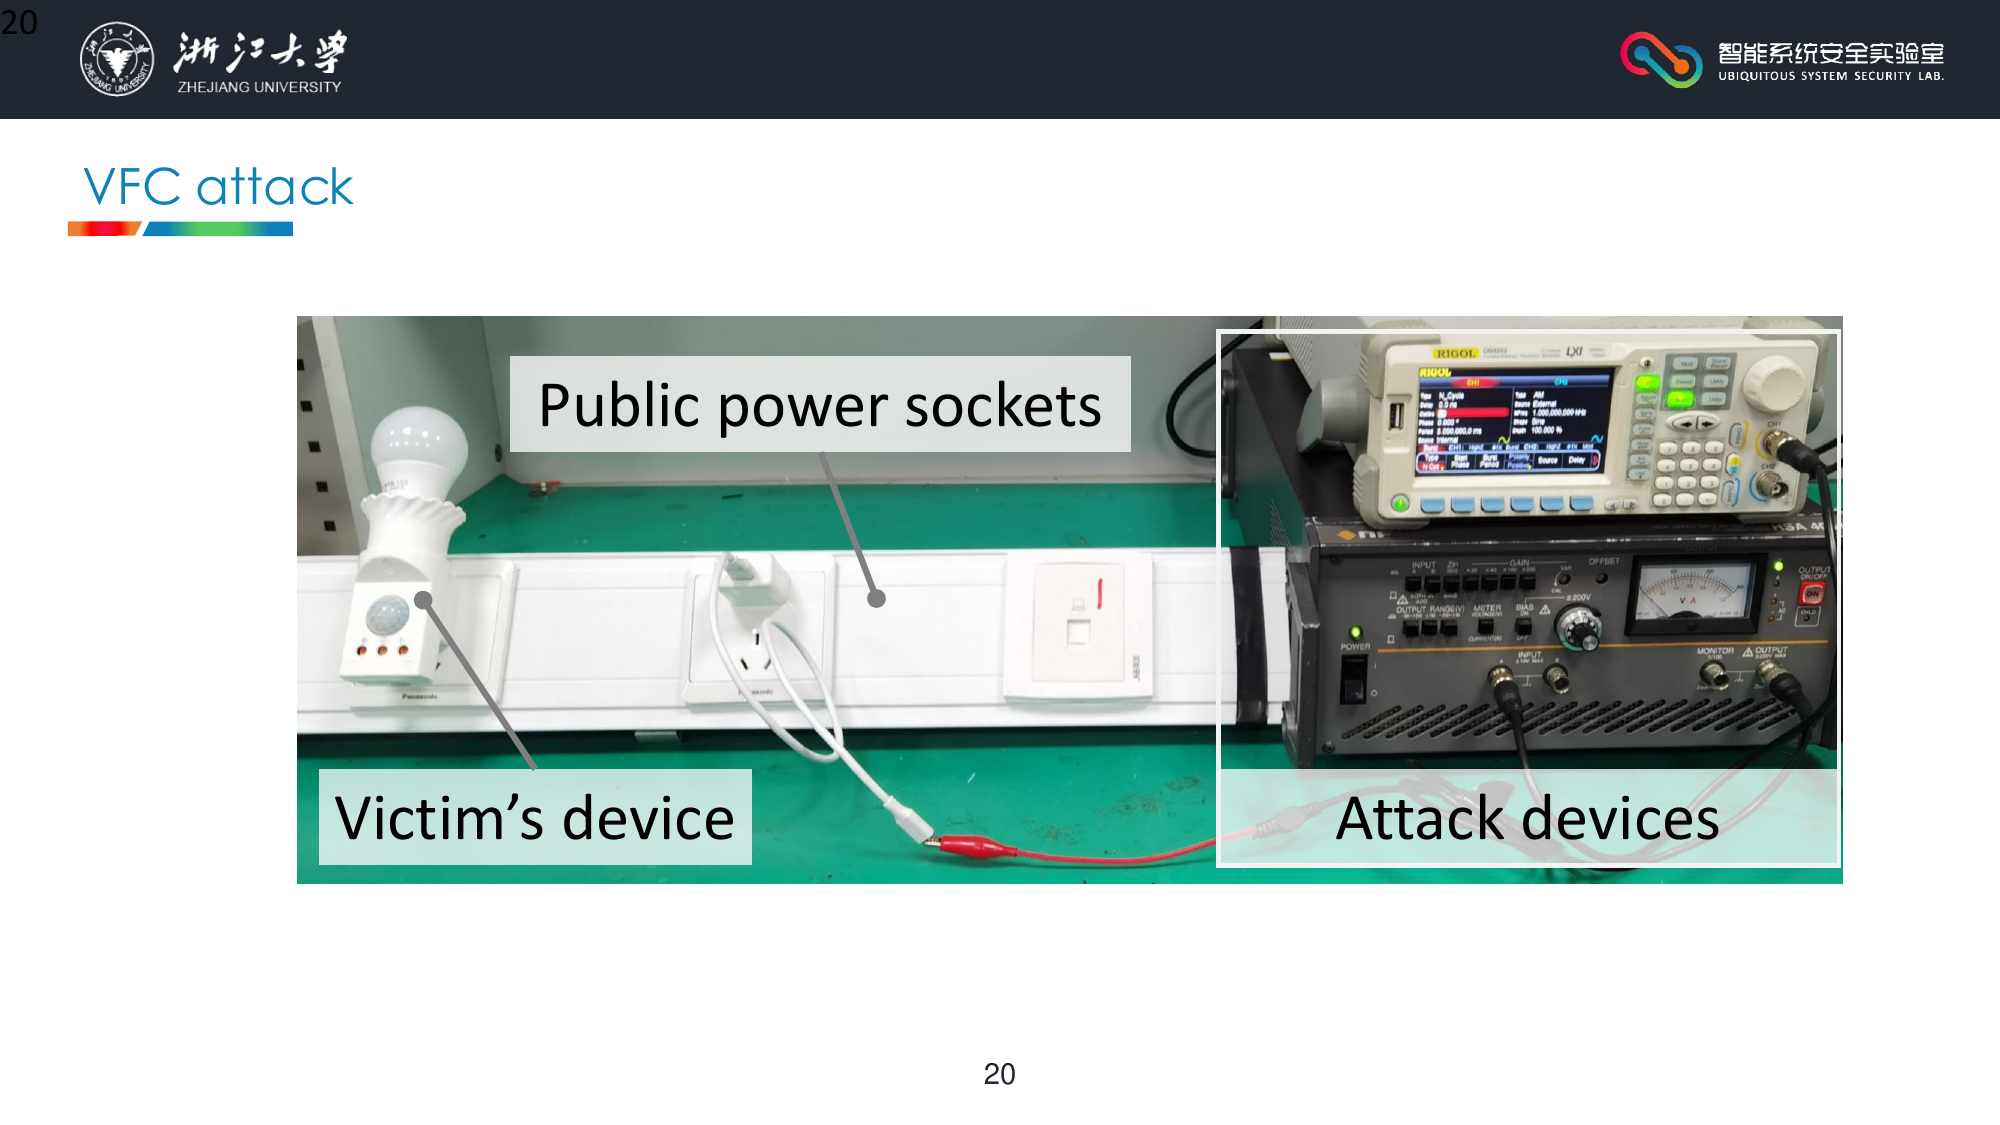}
	\caption{Illustration of across-socket attack against commercial motion detector light. }
	\label{fig: commercialmotionsensor}
\end{figure}

\noindent \textit{(b) 8 tested surveillance cameras.}
\begin{figure}[h]
    \centering
    \includegraphics[width=1\linewidth]{./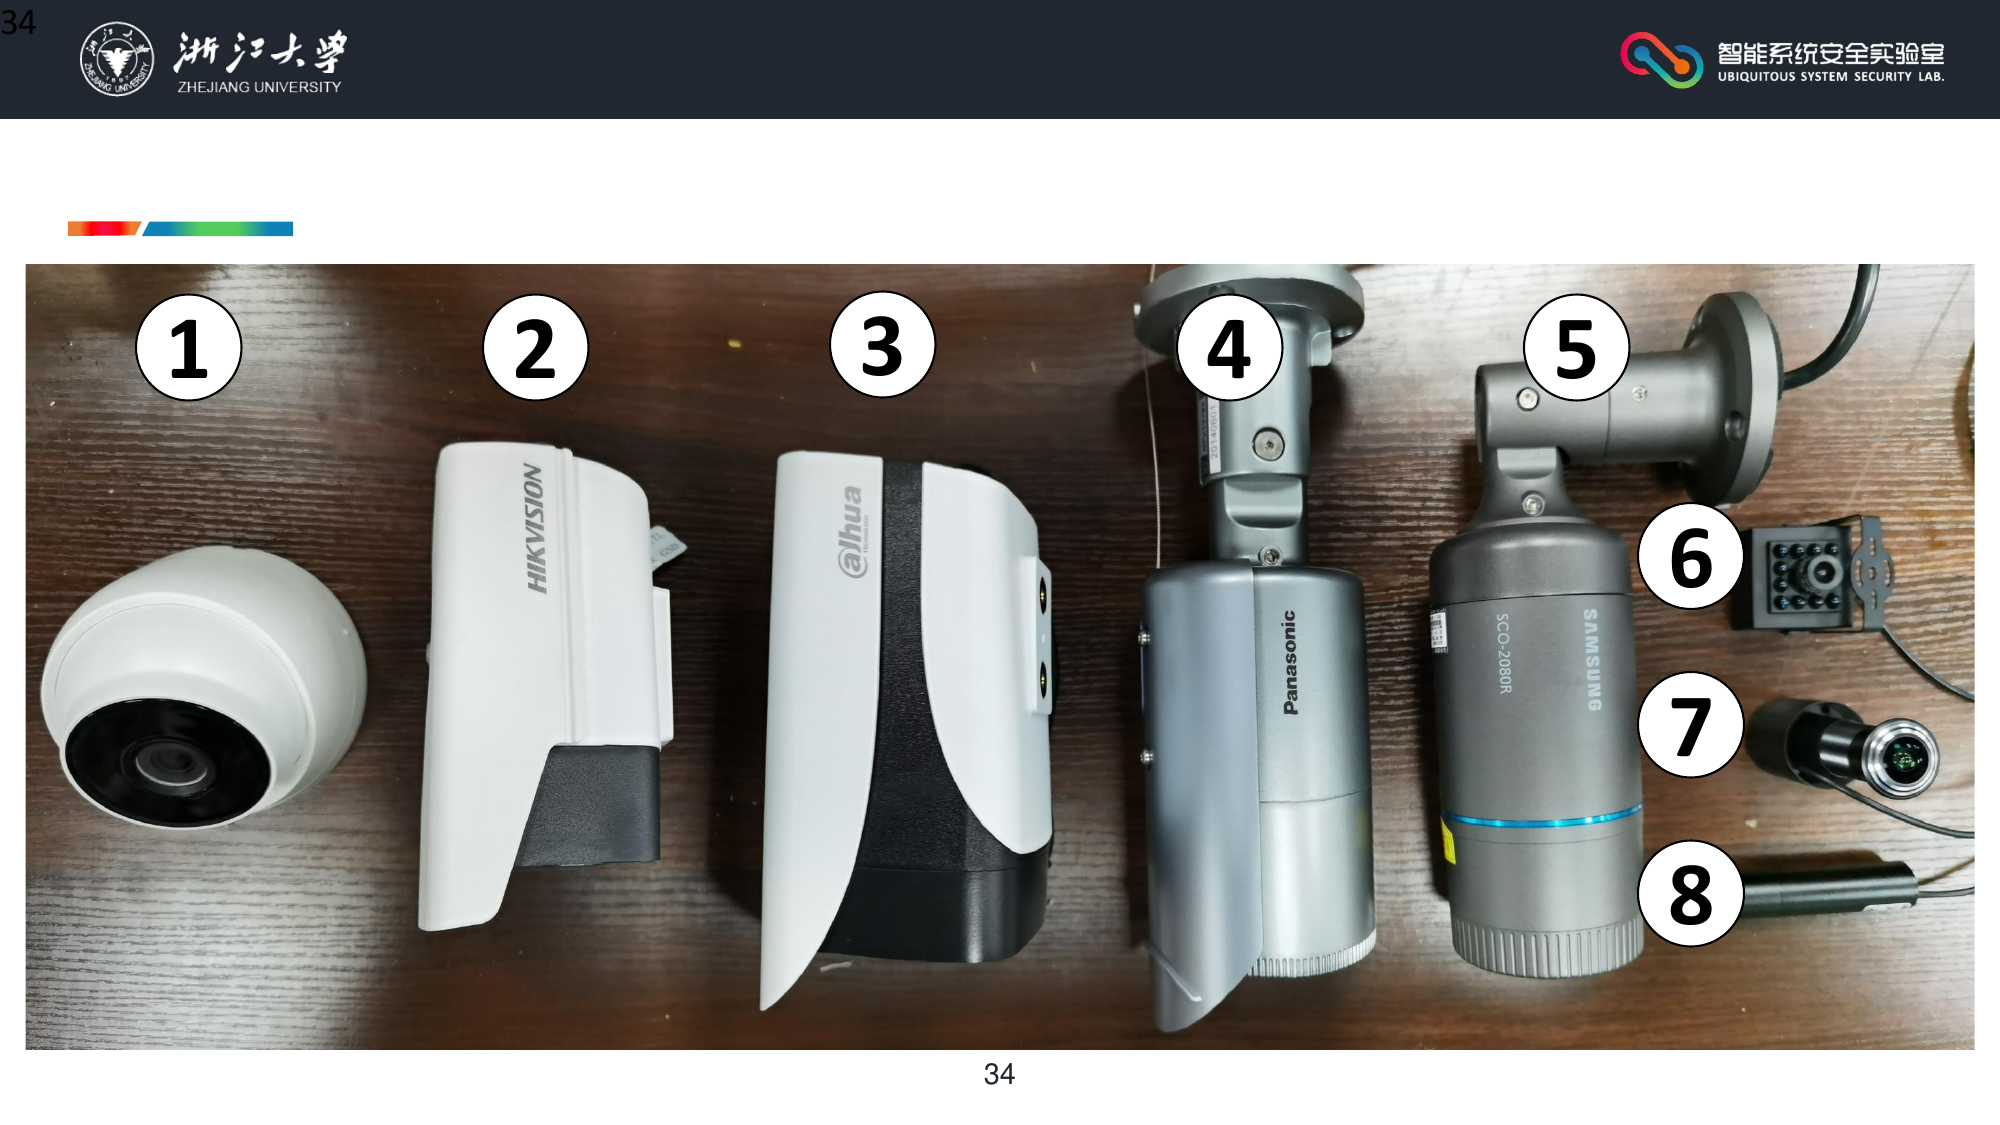}
    \caption{The 8 commercial analog cameras tested in the evaluation: \ding{172} HIKVISION DS-2CE56C3T-IT3~\cite{hikvisiono2024ds2ce56cot}, \ding{173} HIKVISION DS-2CE16G0T-IT3~\cite{hikvisiono2024ds2ce16d0t}, \ding{174} DH-HAC-HFW1200M-I2~\cite{dahua2024dhhac}, \ding{175} Panasonic WV-CW314LCH~\cite{panasonic2024wvcw314lCH}, \ding{176} SAMSUNG SCO-2080RP~\cite{samsung2024sco2080r}, \ding{177} SONY CCD673-1200, \ding{178} SONY CCD-1200, and \ding{179} SONY IMX323 ~\cite{sony2024imx323}.}
    \label{fig: eval_camera_list}
\end{figure}

% \noindent \textit{(c) Illustration of controlled stripes on captured images.}
% \begin{figure}[h]
%     \centering
%     \includegraphics[width=0.8\linewidth]{./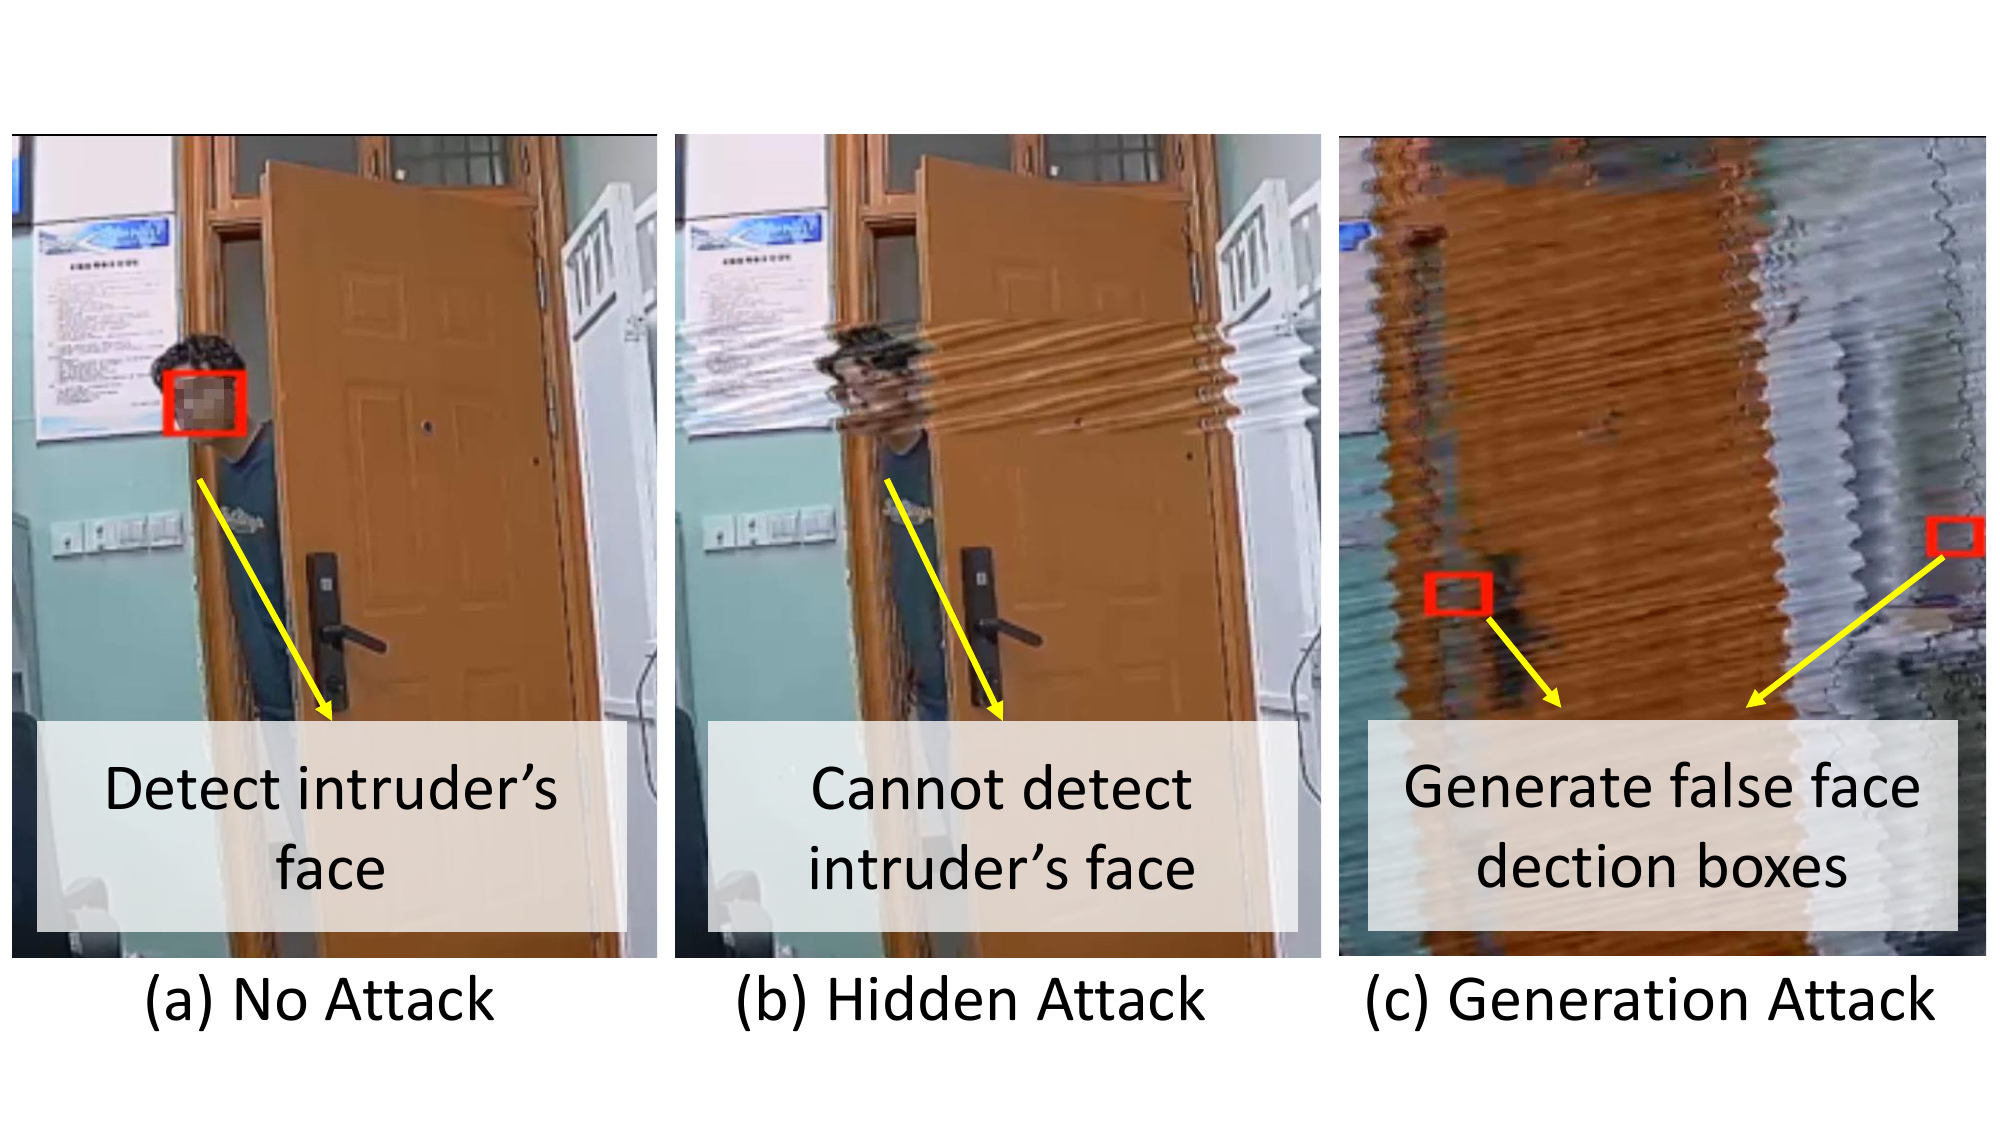}
%      \caption{Attack examples. (a) No attack: the face detection model (Facenet~\cite{schroff2015facenet}) can detect the intruder's face with a red box. (b) Hidden Attack: the narrow-width stripes obscure the intruder's face, making the face detector fail to detect it. (c) Generation Attack: the detector mistakenly detects two faces when no one is on the scene.}
%     \label{fig: result_camera_controlledstripes}
% \end{figure}

\noindent \textit{(c) Illustration of attack scenarios against microphones, including broadcasting, remote conference, and live broadcast.}
% \textit{(d) Illustration of attack scenarios against microphones.}
\begin{figure}[h]
	\centering
	\includegraphics[width=1\linewidth]{./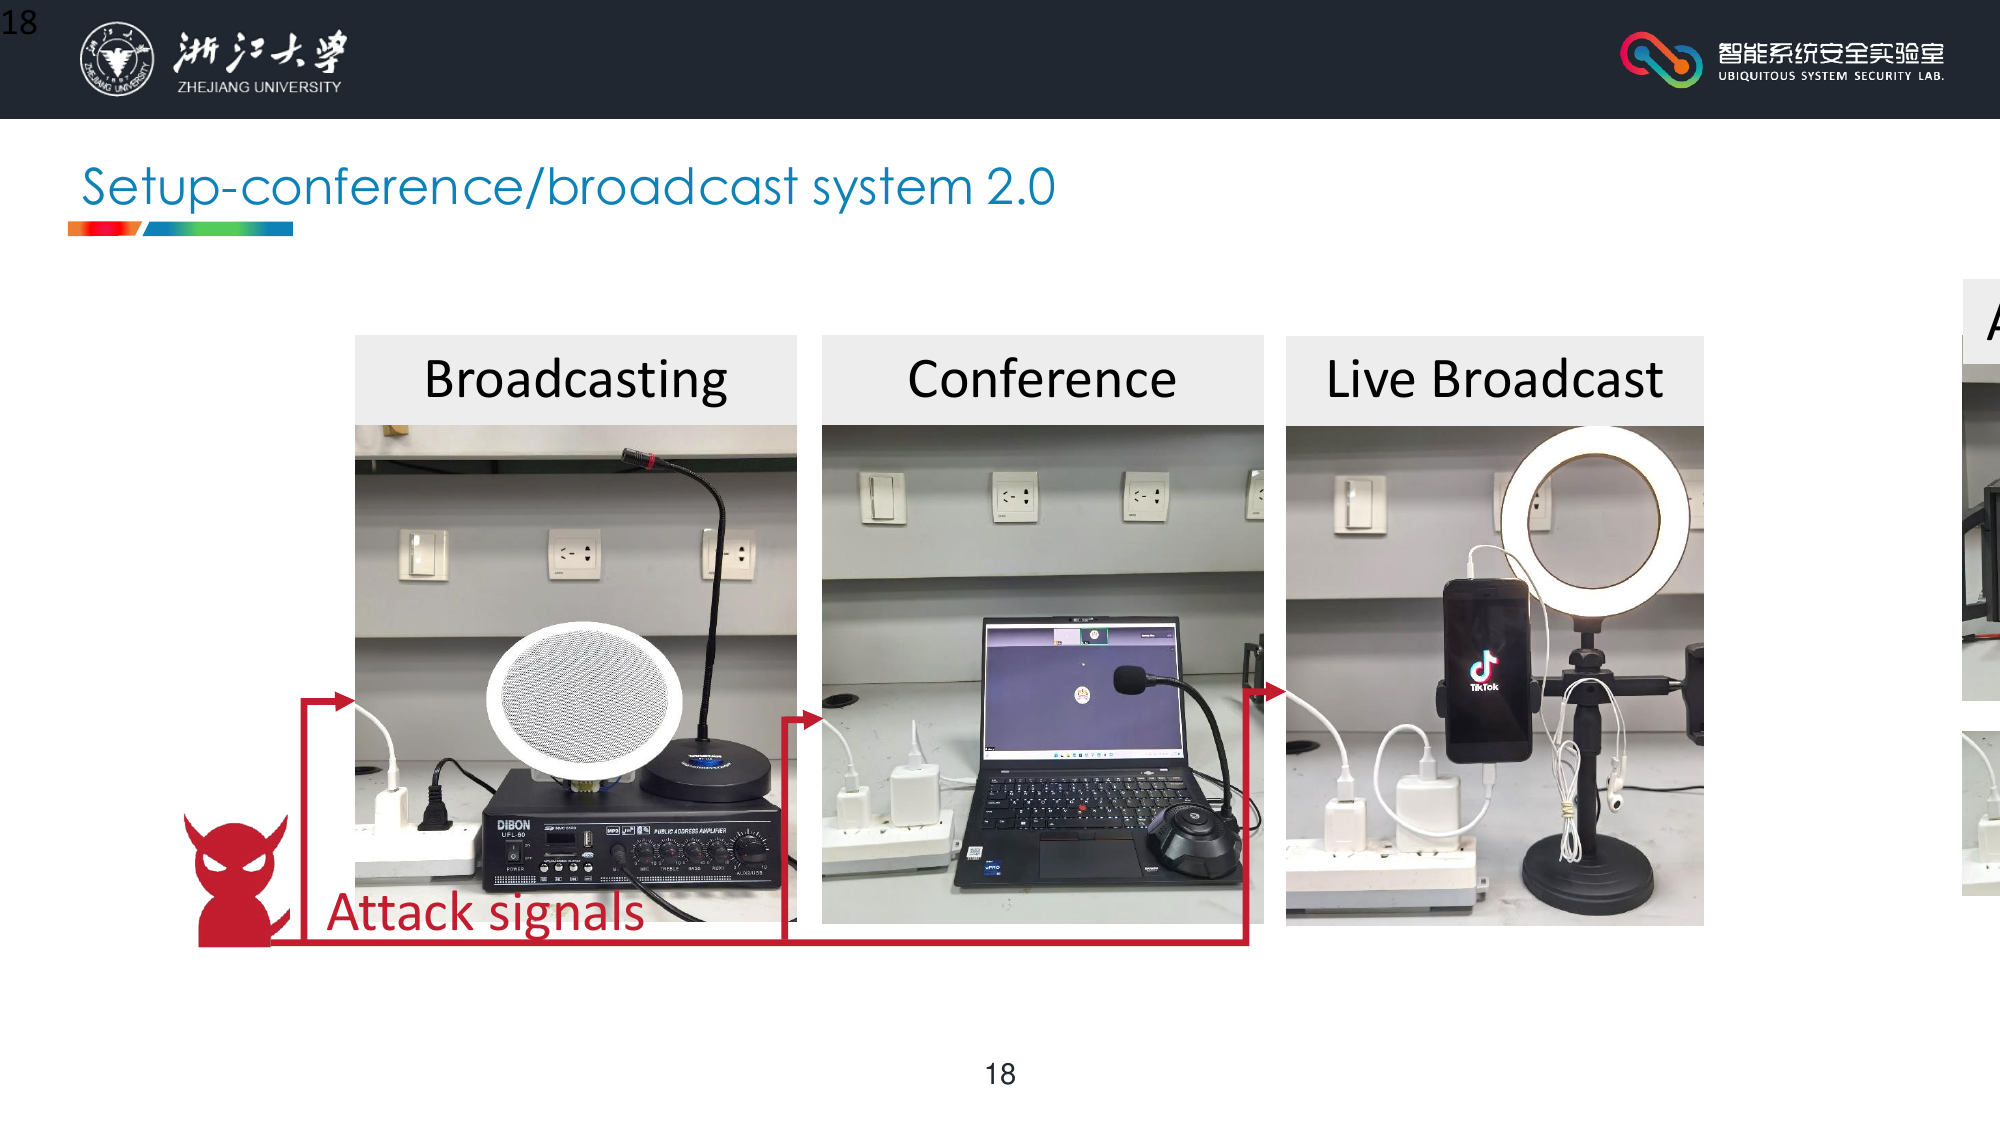}
	\caption{Illustrations of broadcasting attack scenarios. The attacker can successfully inject fake voice audio into the public broadcasting system, remote conference system, and live broadcasting system.  }
	\label{fig: setup_mic}
\end{figure}

\noindent \textit{(d) 7 tested commercial microphones are shown in \fig{fig: eval_mic_list}.}
\begin{figure}[h]
    \centering
    \includegraphics[width=0.78\linewidth]{./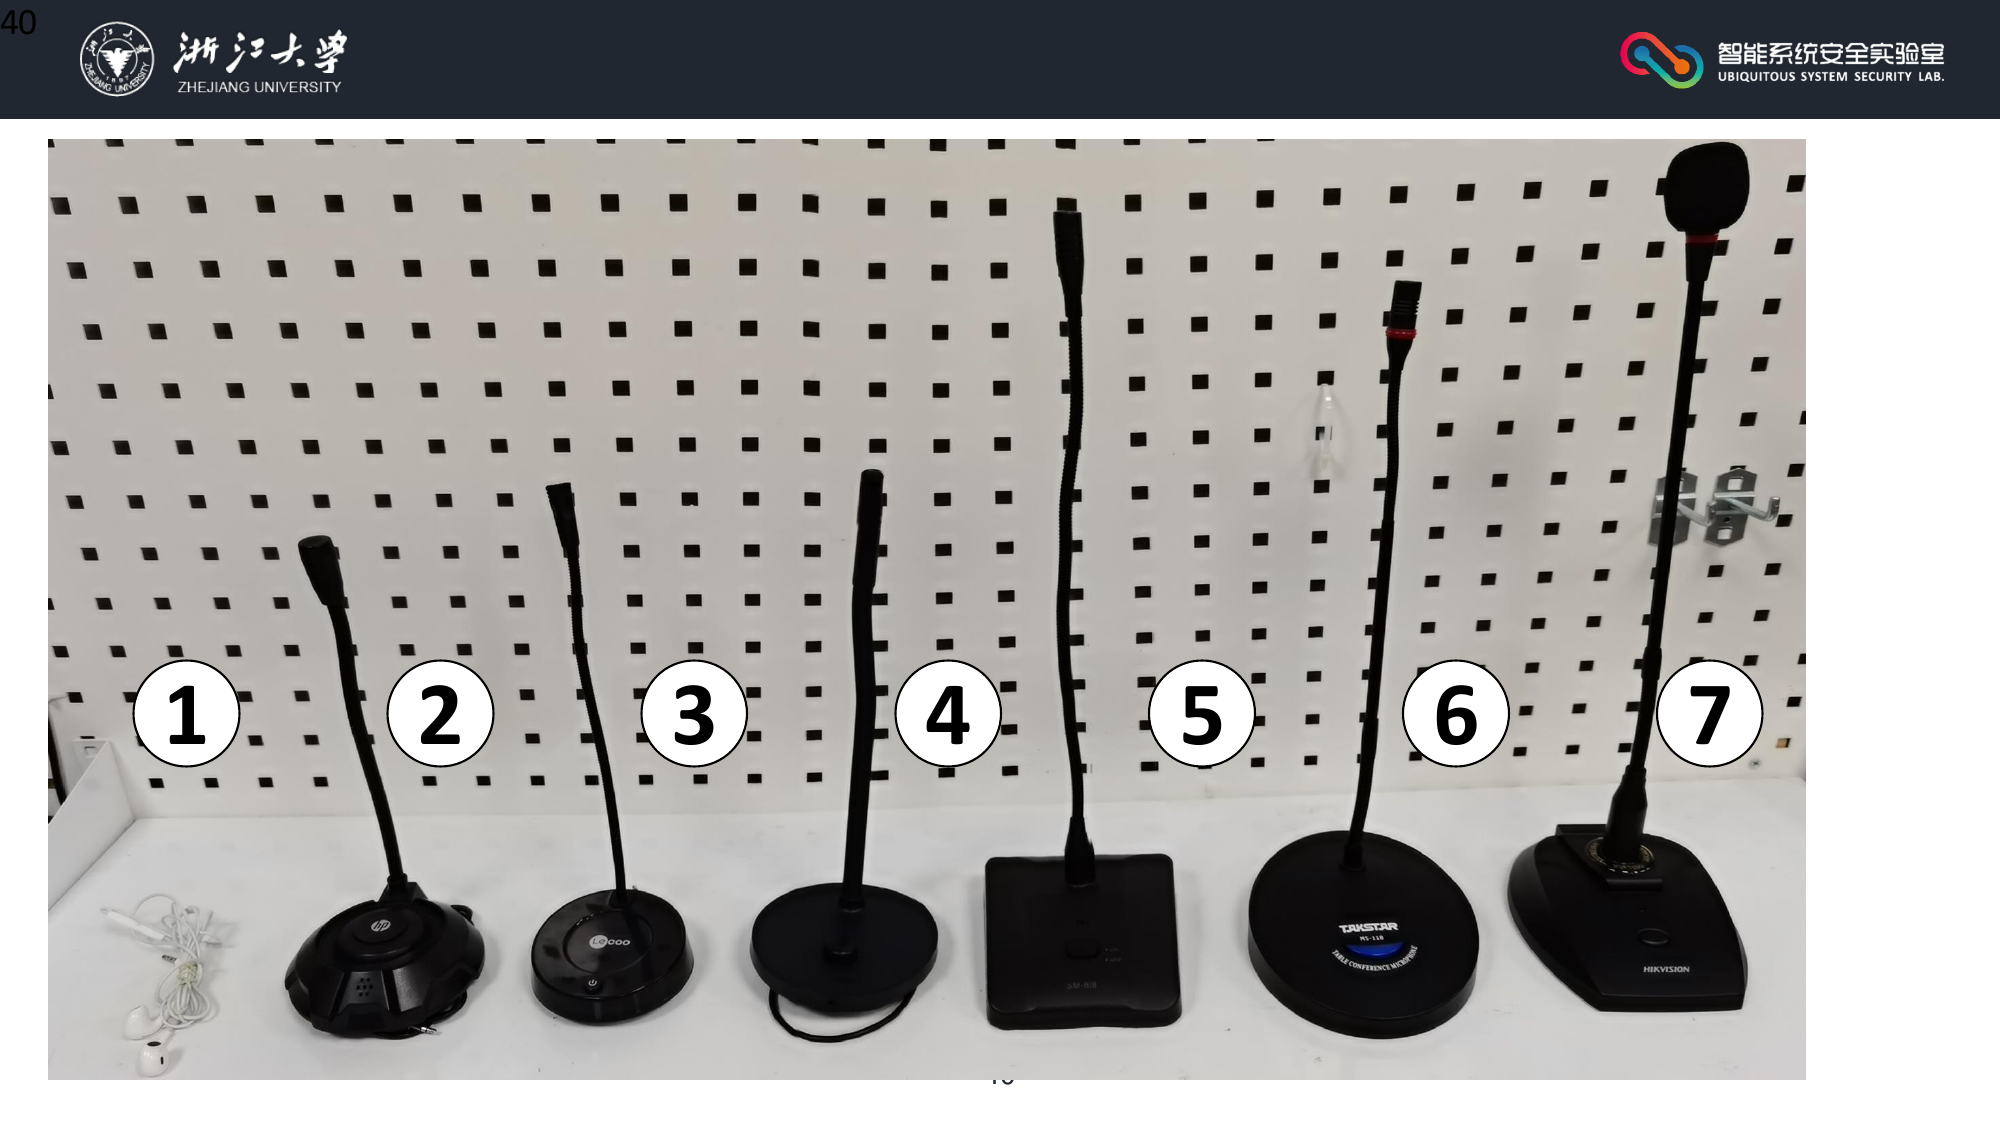}
    \caption{The 7 commercial microphones tested for evaluation: \ding{172} wired earphone HUAWEI AM115~\cite{productz2024huaweimic}, \ding{173} desktop microphone HP DHP-1100l~\cite{jd2024hpmic}, \ding{174} desktop wired microphone Lenovo Lecoo MC01 ~\cite{banggood2024lenovmic}, \ding{175} USB microphone UGREEN CM564~\cite{jg2024ugreen}, \ding{176} broadcast microphone SM88, \ding{177} conference microphone TAKSTAR MS-118~\cite{takstar2024ms118}, \ding{178} conference microphone HIKVISION DS-KAU30HG-M~\cite{jd2024ds-kau30hg-m}.}
	\label{fig: eval_mic_list}
\end{figure}

% \noindent \textit{(e) Other detection results are shown in \fig{fig: eval_yolov_otherresults}.}
% \begin{figure} [h]  
% 	\centering
%  	% \setlength{\abovecaptionskip}{-0.05cm}
%         \subfigure[Facenet Results.]{
% 		\includegraphics[height=0.39\linewidth]{./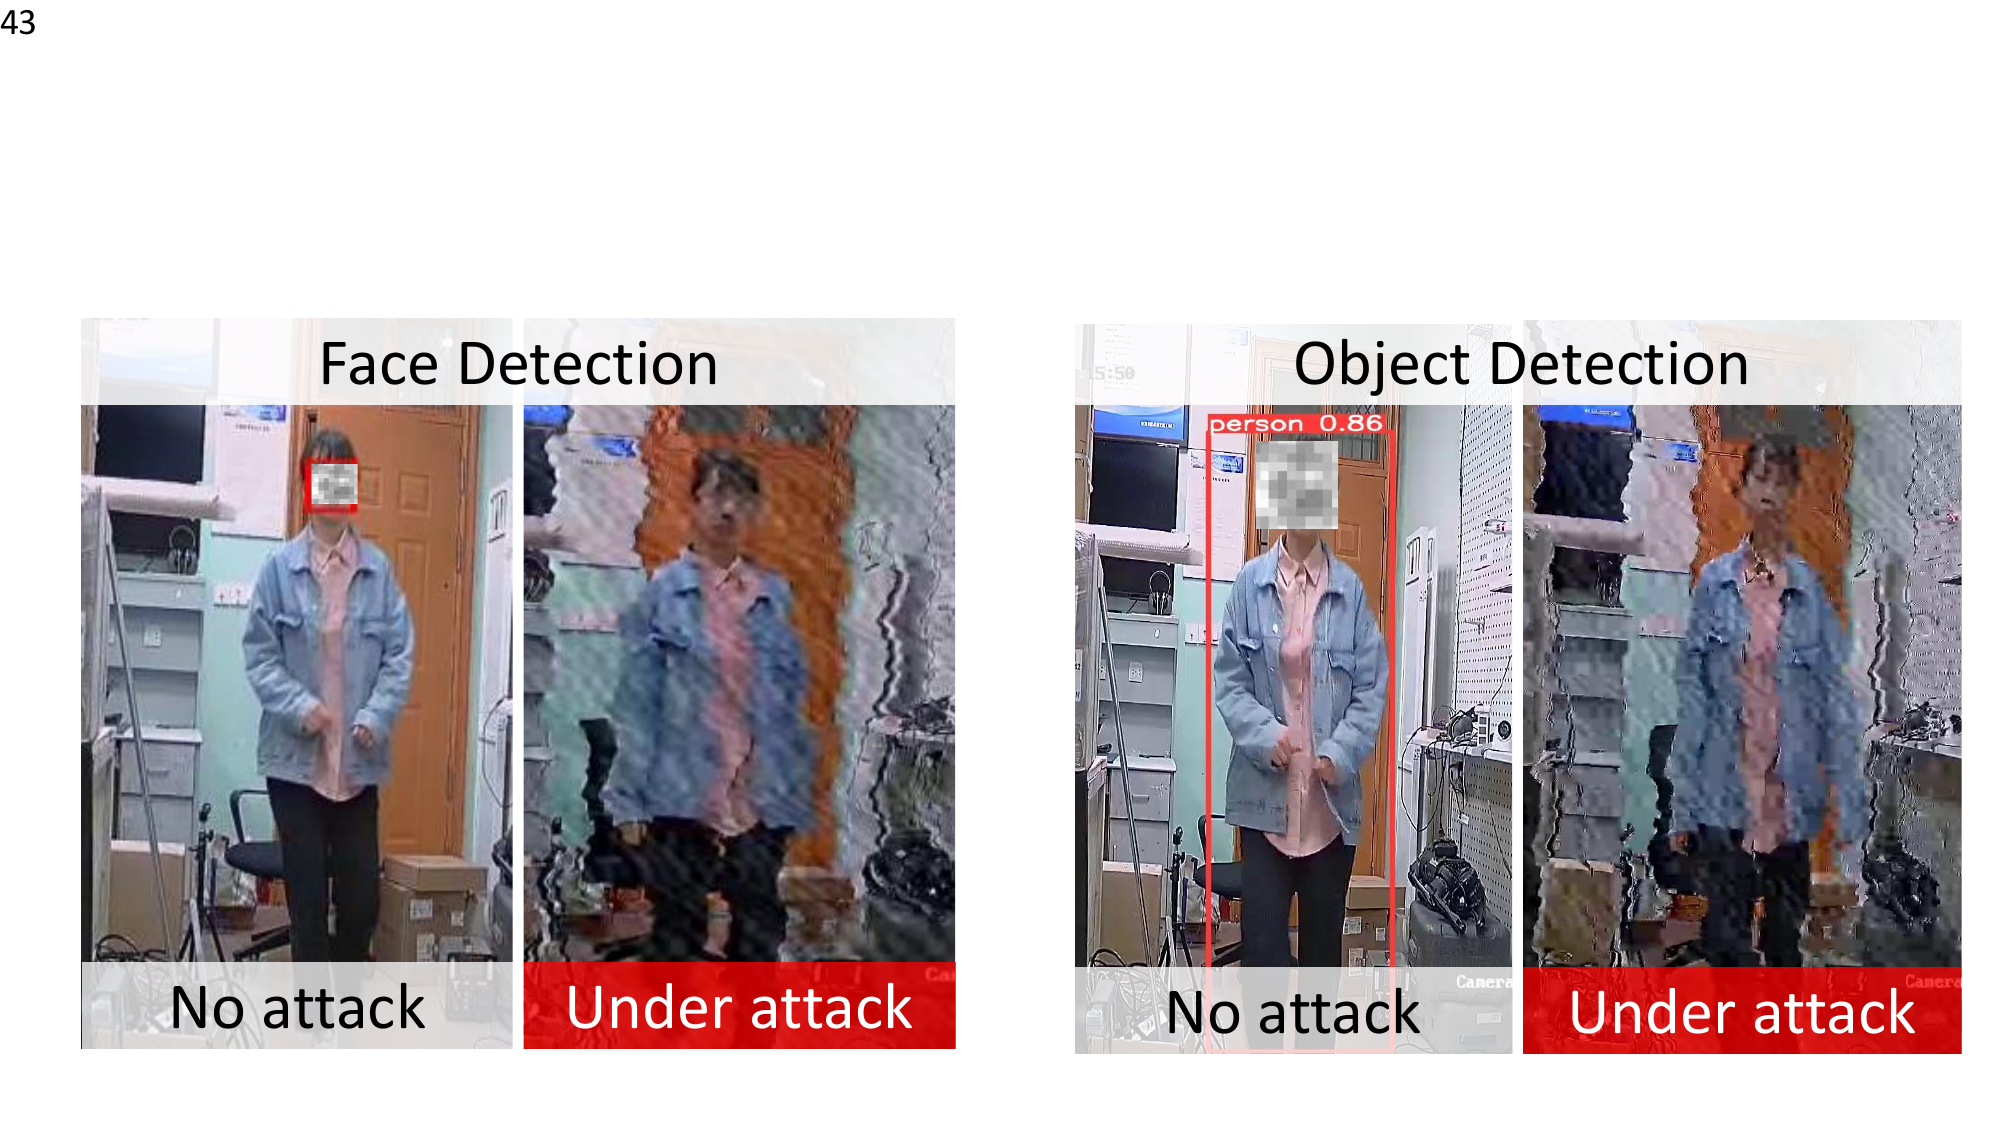}\label{fig: eval_facenet}
% 	}\hspace{-2ex}
%         \subfigure[Yolov8 Results.]{
% 		\includegraphics[height=0.39\linewidth]{./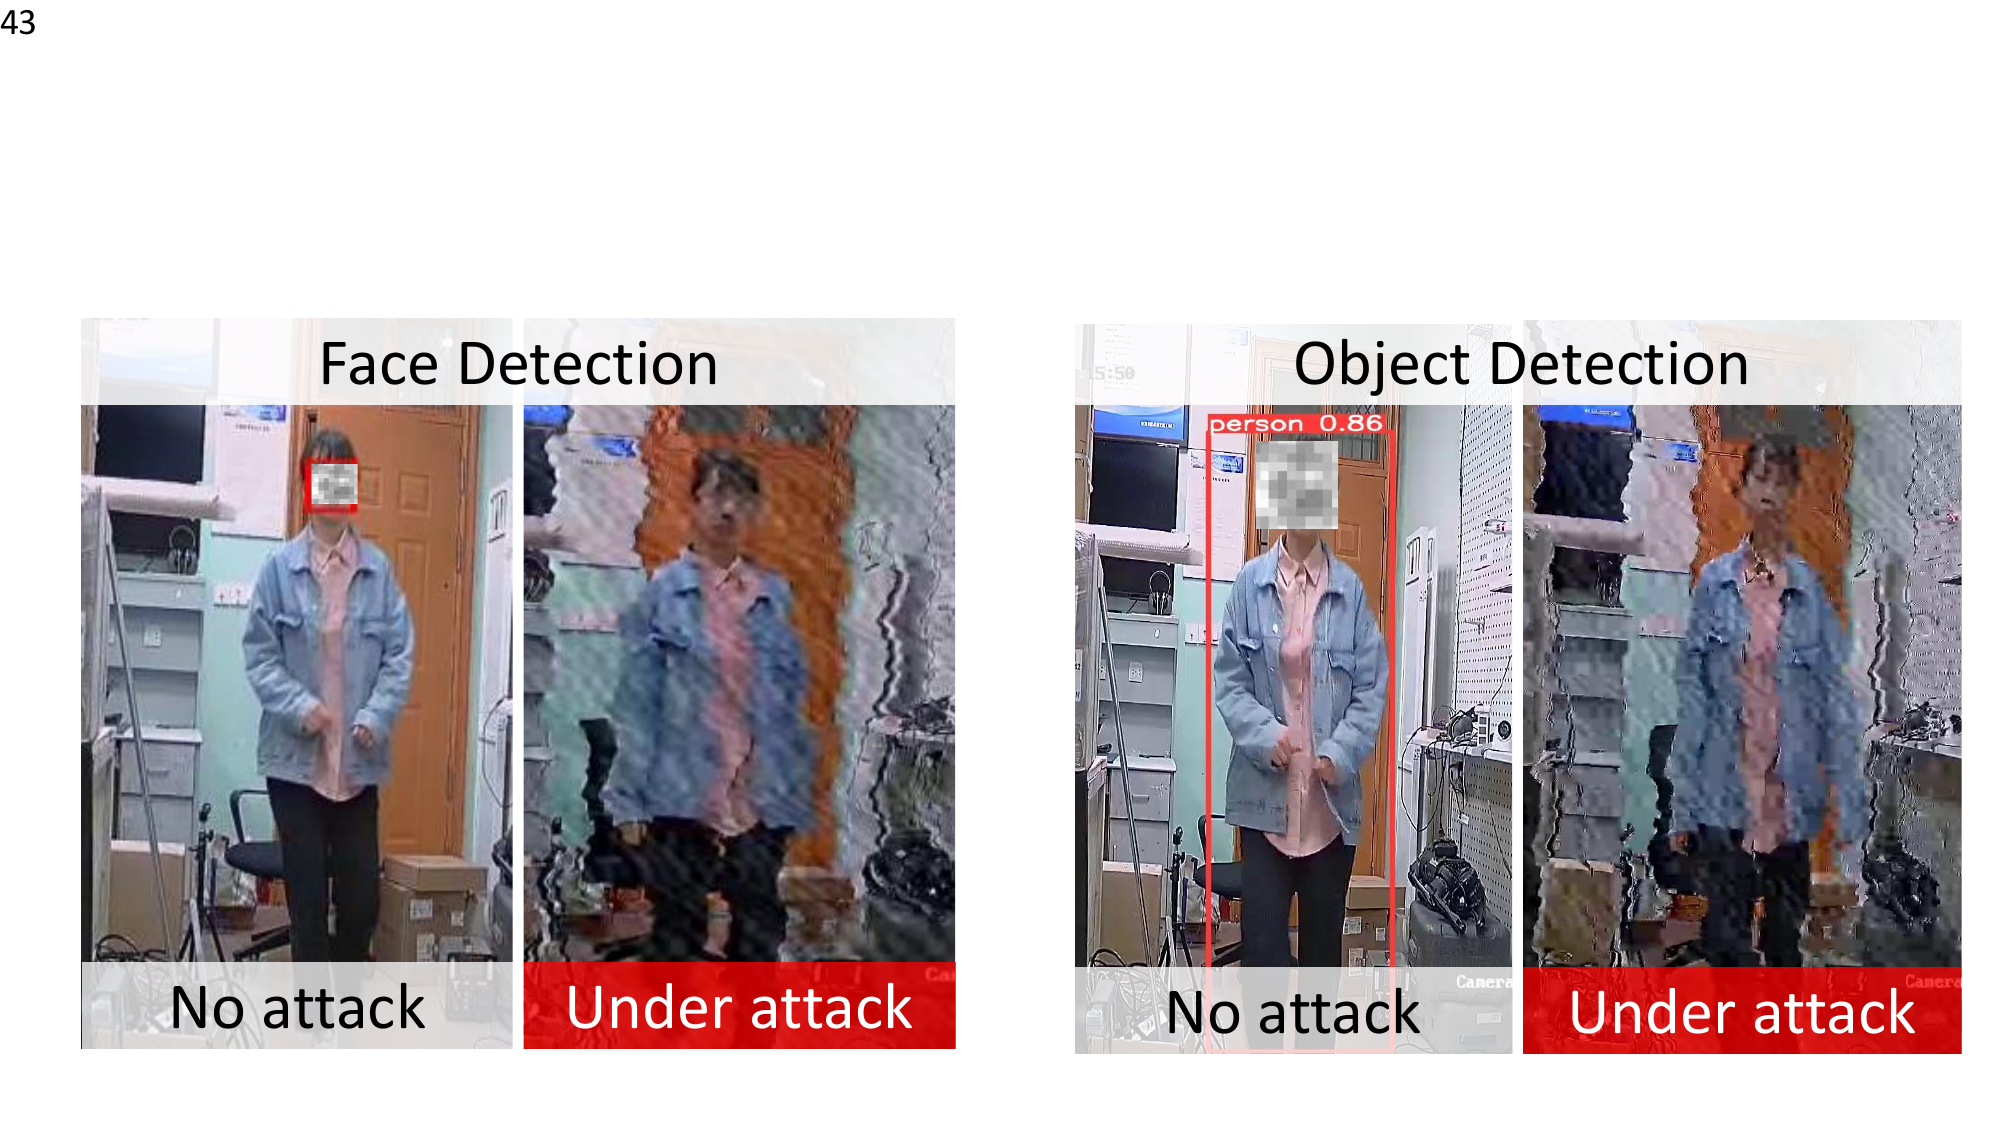}\label{fig: eval_yolov8}
% 	}
% 	\caption{Illustrations of real-world attacks on face detection and object detection by introducing stripes into captured images. (a) The face detection model (Facenet~\cite{schroff2015facenet}) fails to detect the intruder's face from the image captured by the camera under attack. (b) The object detection model (Yolov8~\cite{jocher2023yolov8}) cannot detect the chair in the disturbed image or falsely detect it as a traffic light.}
%     % \vspace{-1.5em}
%  \label{fig: eval_face_object}
% \end{figure}

% \begin{figure}[h]
%     \centering
%     \includegraphics[width=0.8\linewidth]{./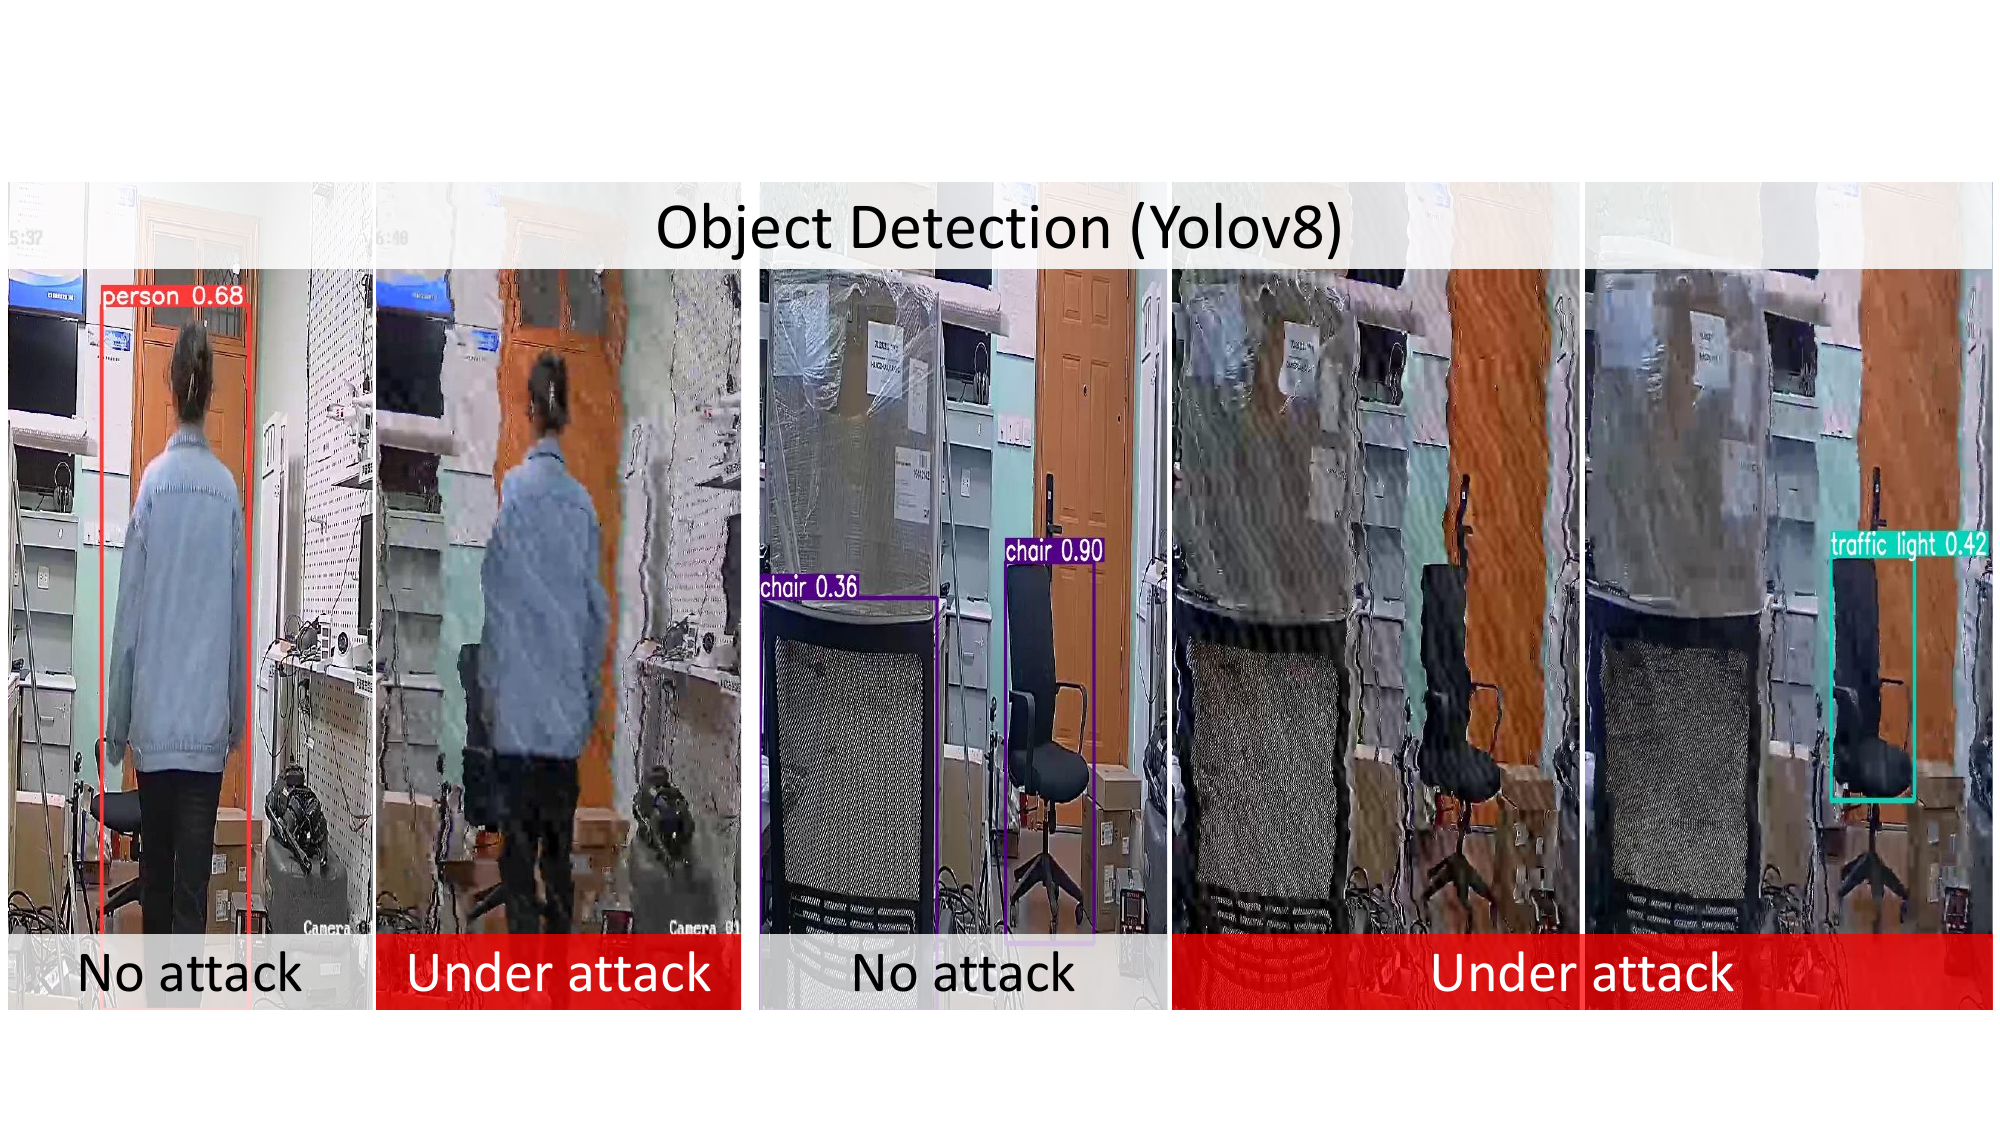}
%     \caption{Illustrations of real-world attacks on object detection (Yolov8) by introducing stripes into captured images. The detection system fails to identify the person, cannot detect the chair in the disturbed image or falsely detect it as a traffic light.}
%     \label{fig: eval_yolov_otherresults}
% \end{figure}

\noindent \textit{(e) The back panel of the household power distribution system and the side view of the system are shown in~\fig{fig: backpanel_and_grid}, and the evaluated noise sources are displayed in~\fig{fig: microgrid_3}.}
\begin{figure}[h]
    \centering
    \subfigure[Back panel.]{\includegraphics[height=0.45\linewidth]{./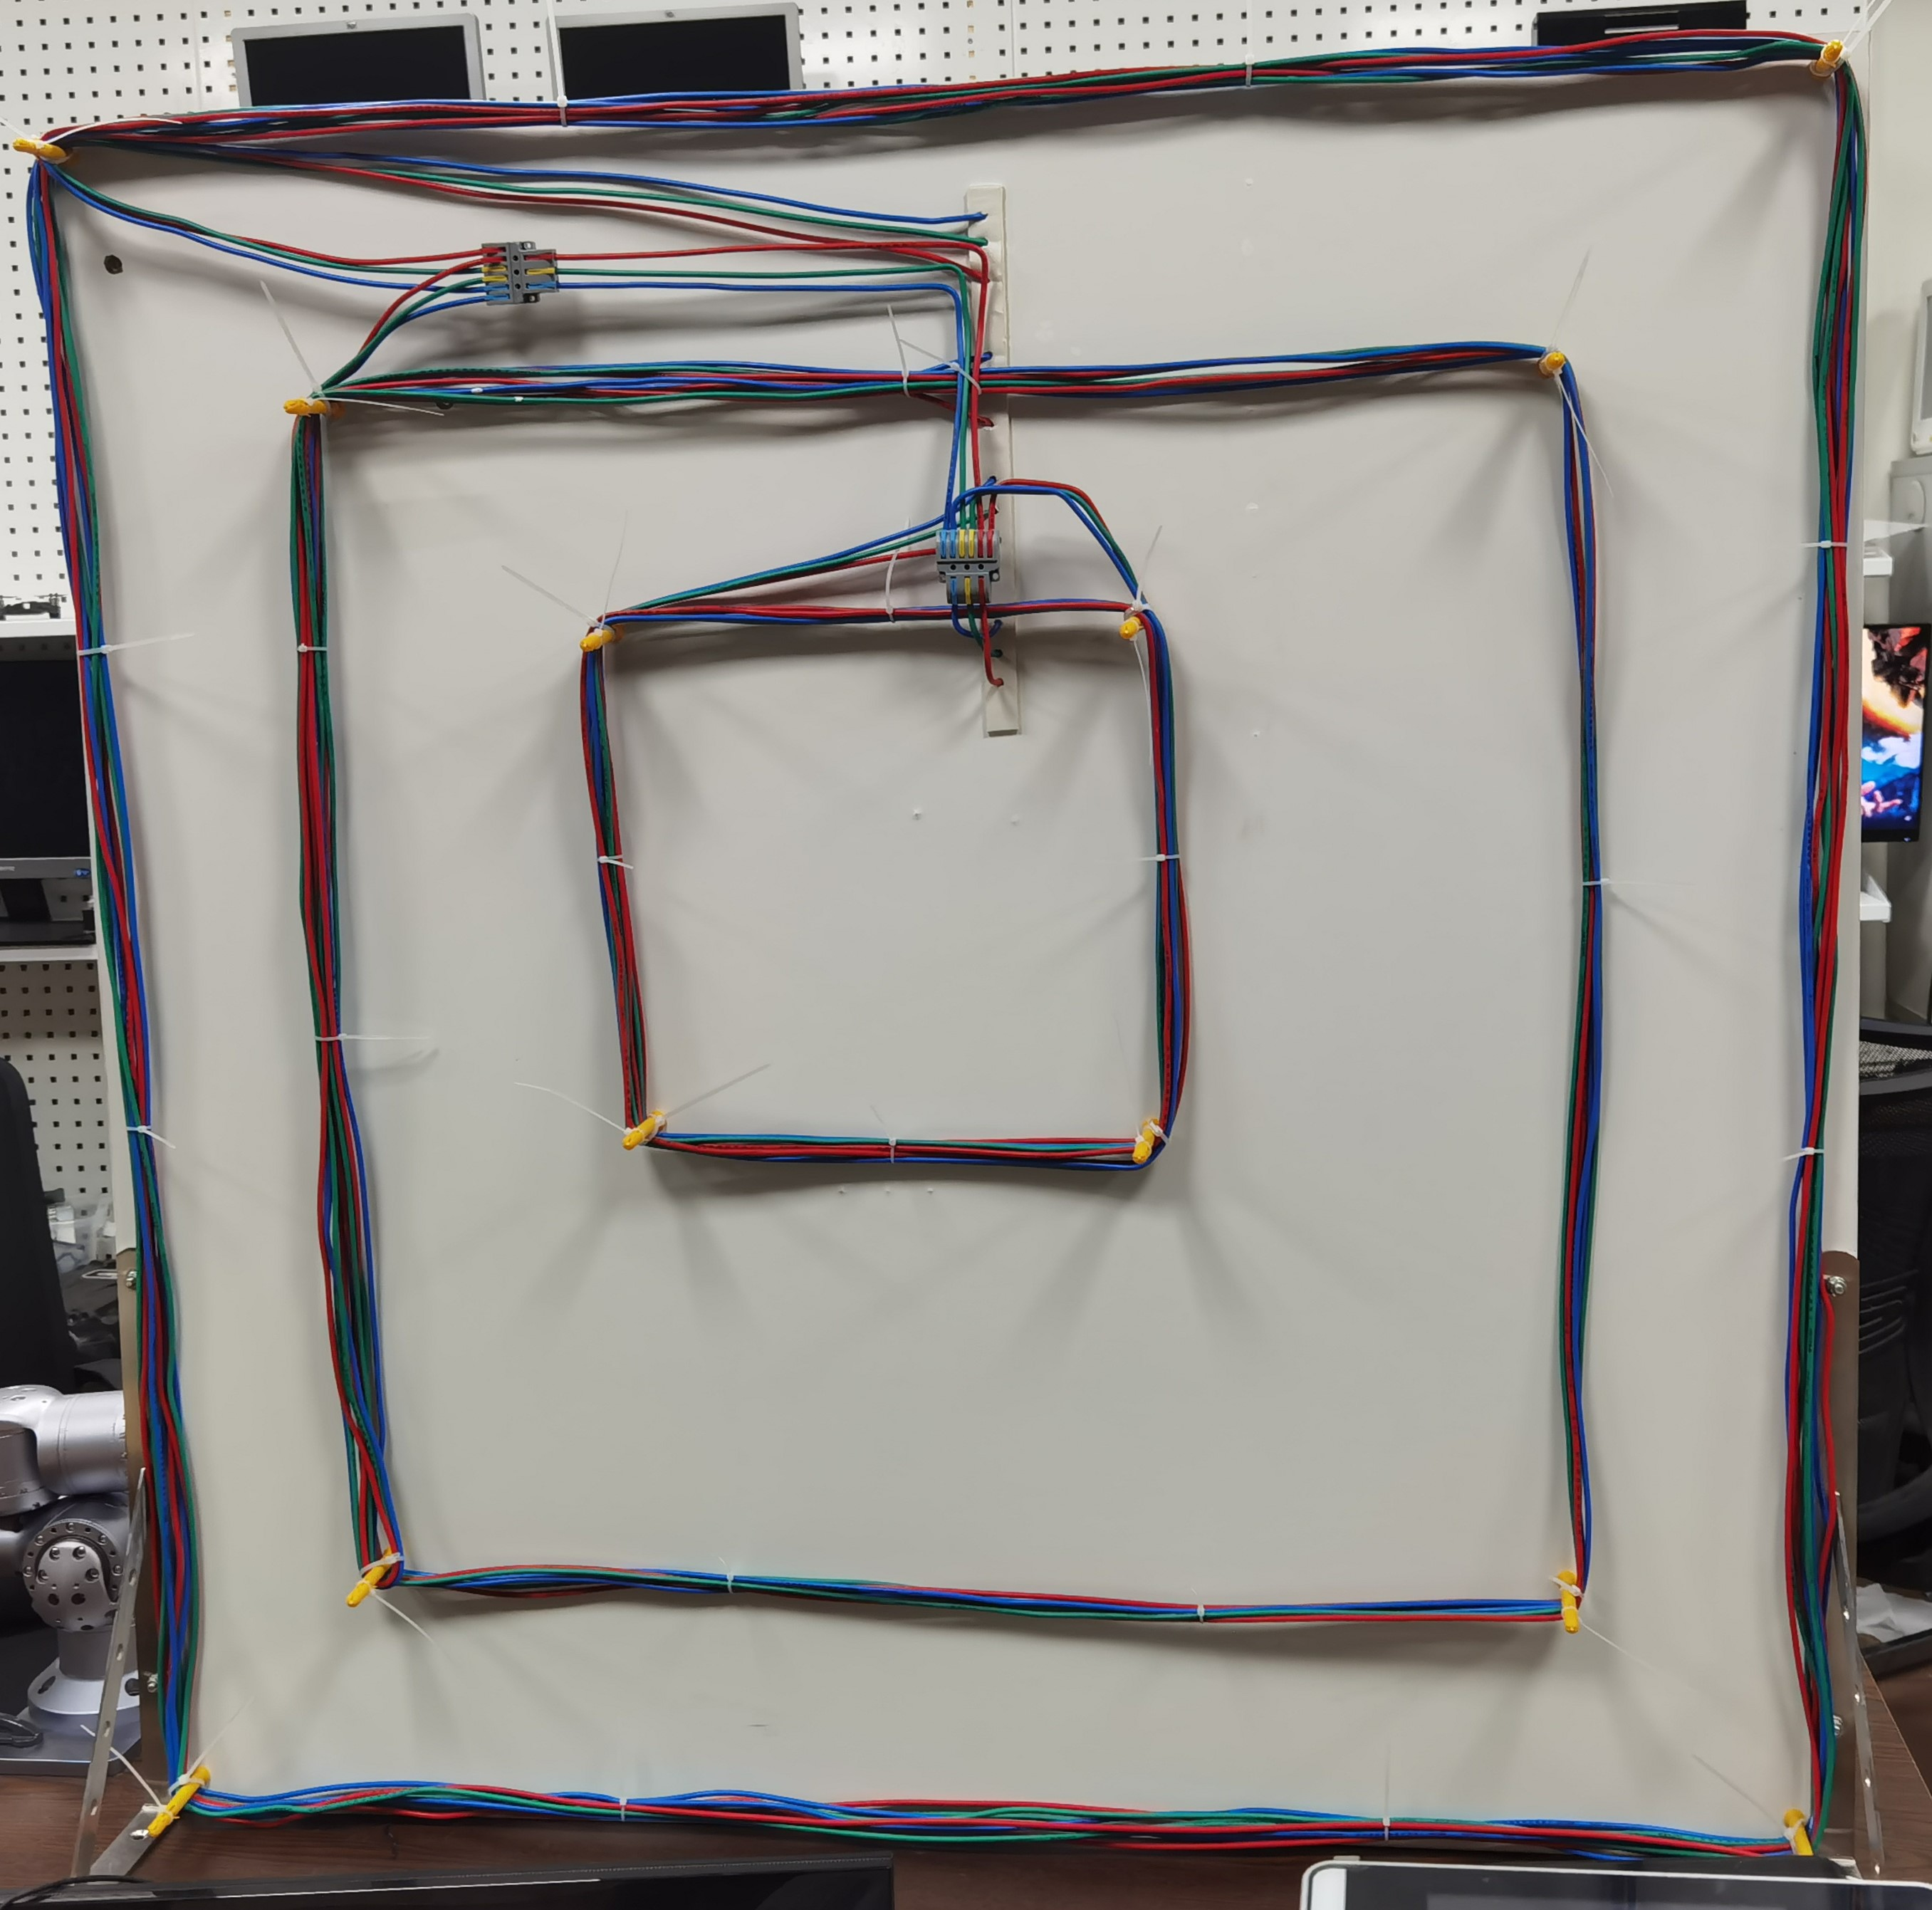}\label{fig: back panel}
	}\hspace{-0ex}
    \subfigure[Part of grid.]{
	\includegraphics[height=0.45\linewidth]{./figures/part of grid.jpg}\label{fig: part of grid}
	}
    \caption{\blue{Illustration of the back panel of the household power distribution system (left) and the side view of the system (right).}}
% \vspace{-6pt}
\label{fig: backpanel_and_grid}
\end{figure}

\begin{figure}[h]
    \centering
    \includegraphics[width=0.8\linewidth]{./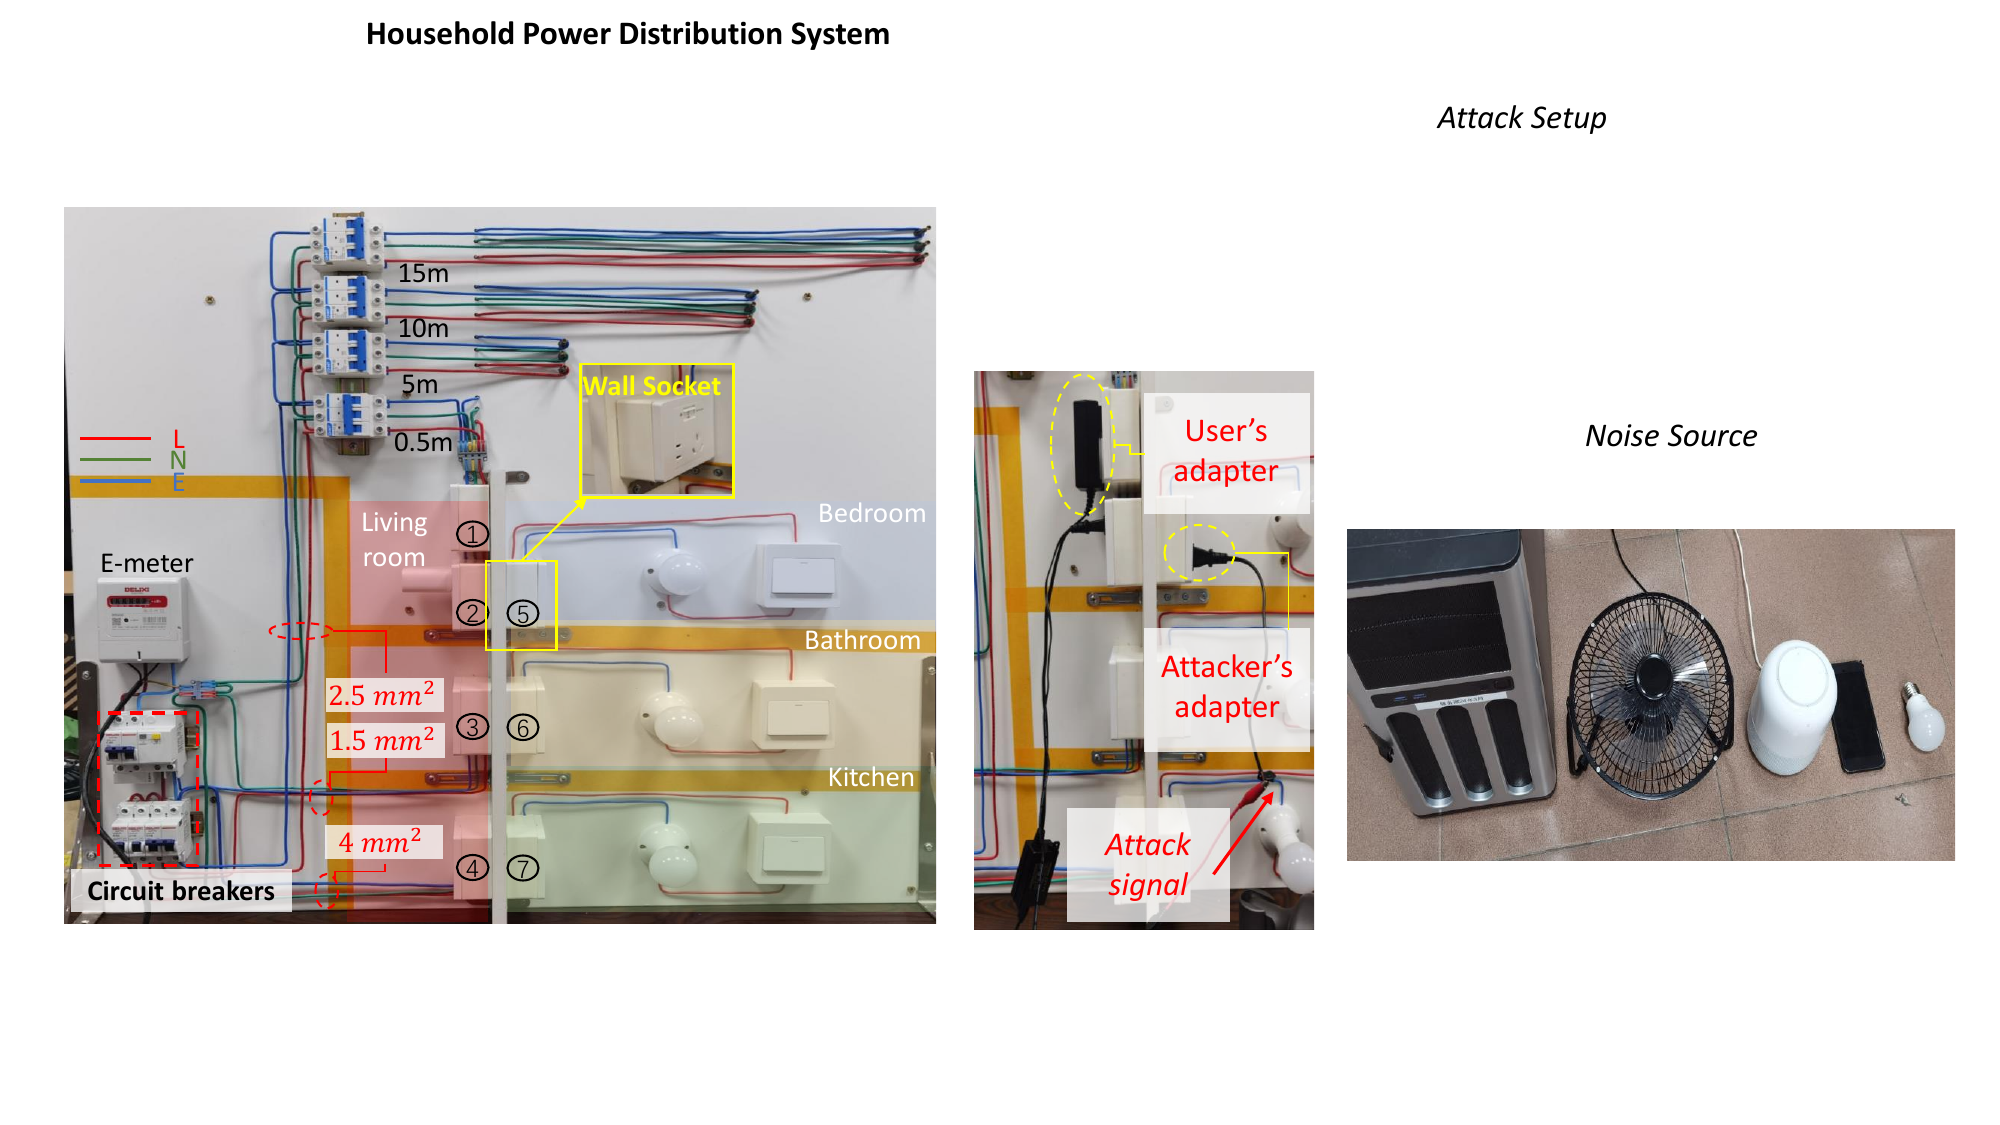}
    \caption{Illustrations of noise sources.}
    \label{fig: microgrid_3}
\end{figure}

% The results are shown in~\fig{fig: result_camera}: (a) the red box in~\fig{fig: result_camera}(a) demonstrates the face detector can successfully detect the intruder's face before conducting the~\alias attack. (b)~\fig{fig: result_camera}(b) shows width-limited stripes blur the intruder's face, leading the detector to fail to detect. These controlled stripes include additional three parameters: setting the signal delay to 5 ms, the signal interval to 40 ms, and the signal cycle number to 1600. (c)~\fig{fig: result_camera}(c) shows that two faces are created in the glitch image. We envision that the above attack outcomes may mislead surveillance systems in various scenarios, such as airports, supermarkets, residences, etc., and damage social security.

\subsection{\textsc{Systemization of Coupling \& Converting Stage}} \label{sec: appendix_coupling&converting}
In this subsection, we elaborate on how the coupling \& converting stage in~\fig{fig: principle_main} of Sec.~\ref{sec: energy_conversion_model} works according to ~\fig{fig: principle_specific}. The coupling stage occurs mainly between the parallel signal and GND lines, and the converting stage occurs mainly in the circuit of the sensors. 
% Our attack signal is converted to a common mode (CM) current through the coupling stage. The common mode (CM) current forms a differential mode (DM) voltage under the converting effect.

\begin{figure*}[th]
    \centering
    \includegraphics[width=0.8\linewidth]{./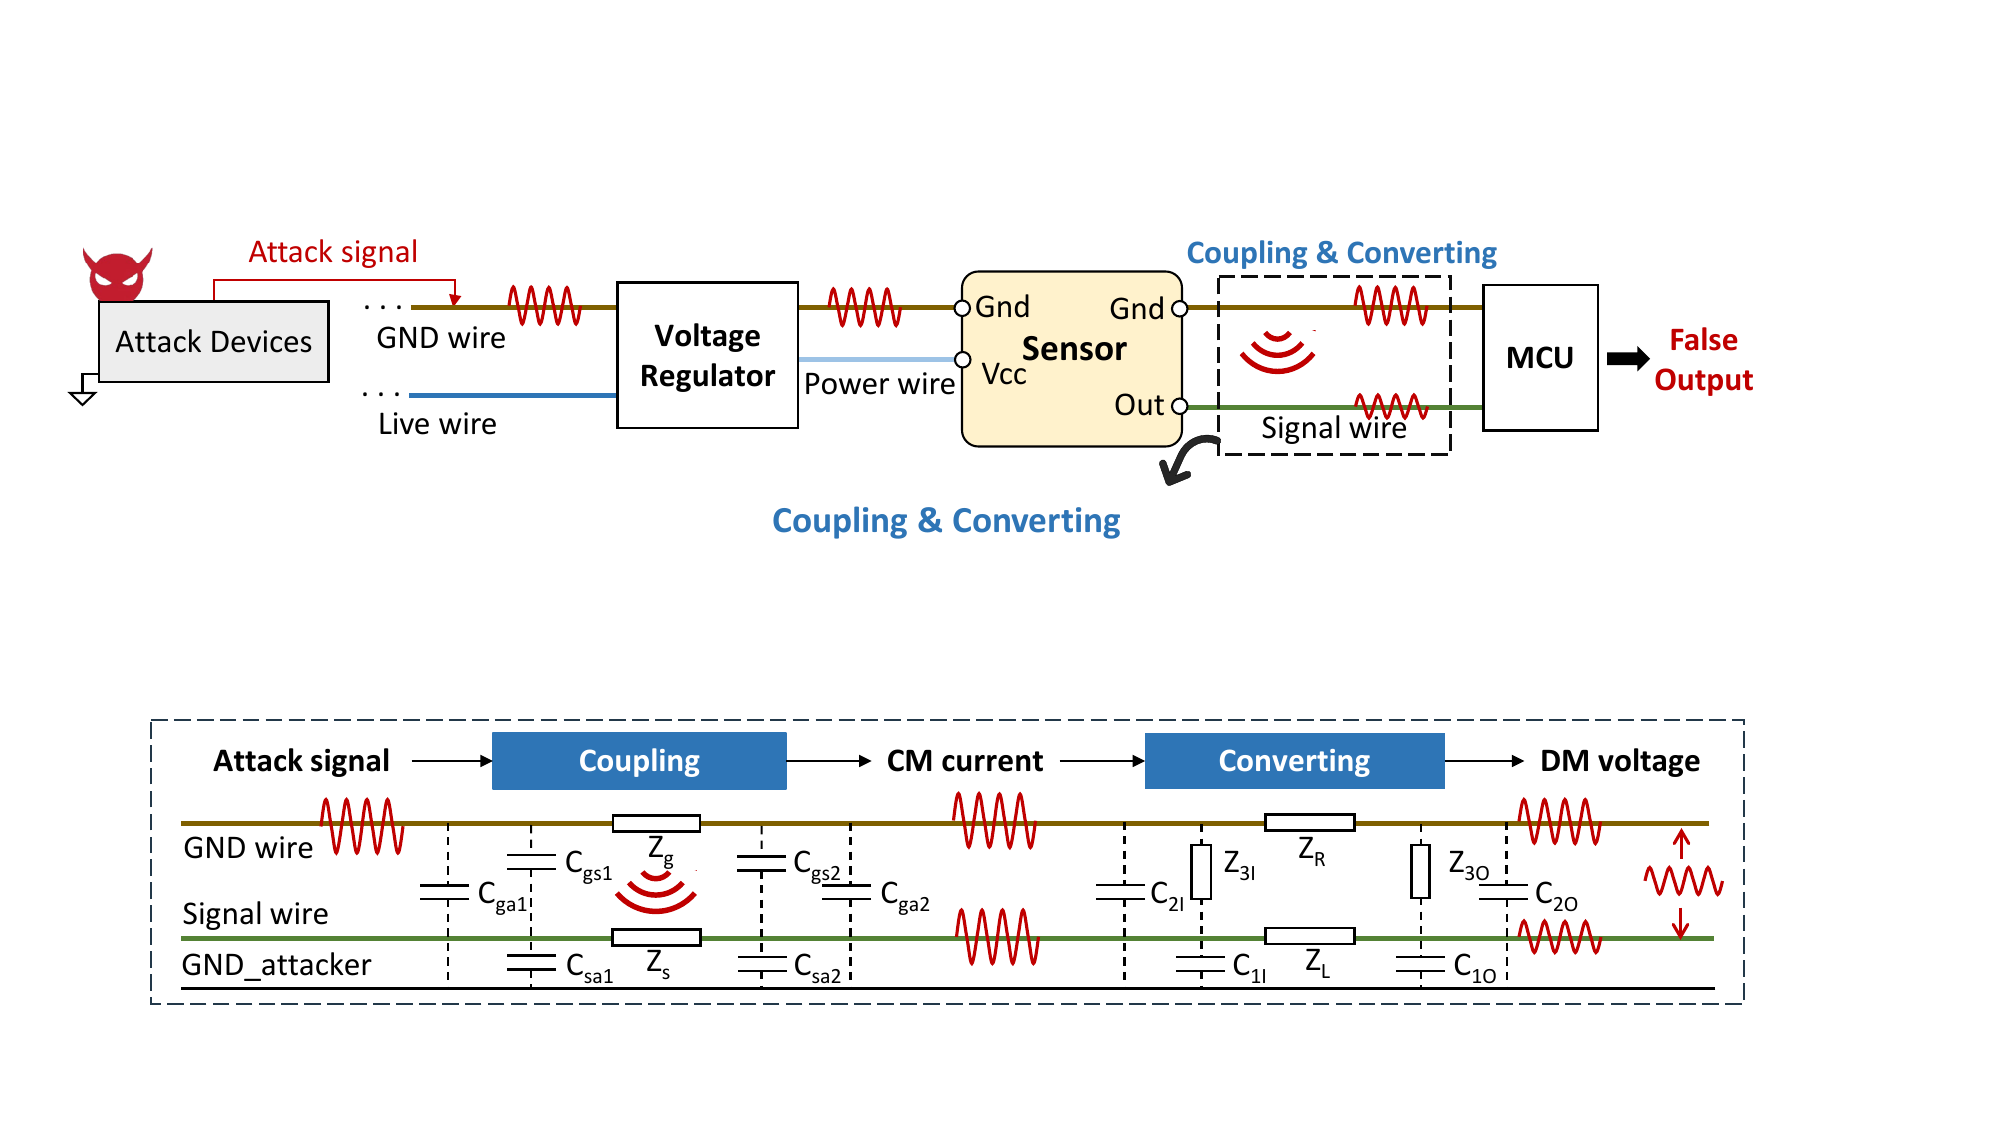}
    \caption{Principle of coupling \& converting stage. We use simple capacitors, impedance loads, and transmission lines to model the energy conversion processes. The wired signal initially radiates from the GND and couples to the signal lines through parasitic capacitors and subsequently generates CM current. Then the CM current is converted into a DM voltage across the output load due to the electronic imbalance.}
    \label{fig: principle_specific}
\end{figure*}

Specifically, the first stage is the coupling stage, in which the GND wire acts as a signal carrier and a potential antenna, coupling the attack signal to the nearby parallel signal line through parasitic capacitors~\cite{pcbdesignTI, zumbahlen2011linear}.
The left circuit in~\fig{fig: principle_specific} shows a schematic of a portion of the transmission lines within the victim device. It is simplified by impedance and transmission lines.
Here, $GND\ wire$ and $GND_{attacker}$ denote the referenced signal GND wire of the victim device and attack device, respectively. The attack signal is applied to the $GND\ wire$. And $signal\ wire$ represents the signal line of the victim device. 
Additionally, $C_{ga}$, $C_{gs}$ and $C_{sa}$ indicate parasitic capacitance between referenced GND and signal lines, while $Z_g$ and $Z_s$ represent the line impedance of the victim device's GND line and the signal line. 

Another parallel stage is the converting stage, where the CM current transforms into a DM voltage due to the electrical imbalance, consequently inducing false measurements for the sensor. 
Similar to the coupling stage, we also use simple impedance and transmission lines to depict the CM-DM conversion model and adopt a group of polynomials to quantize the affecting factor, i.e., the imbalance factor.~\fig{fig: principle_specific} displays a universal electronic circuit, where $C_{1I}$, $C_{2I}$, $C_{1O}$, and $C_{2O}$ are parasitic capacitance between the victim's signal wire and GND line with the attacker's GND, $Z_{3I}$ and $Z_{3O}$ represent the impedance between victim's GND wire and signal wire, $Z_{L}$ and $Z_{R}$ are impedance that is comprised of electronic components on the transmission lines (i.e., the GND line and the signal line).

% 两个阶段看上去很像，有什么区别
Some readers may find that the circuit diagrams for the two stages are similar. But they are actually different. 
% coupling阶段中GND wire和signal wire之间的电容是寄生的，而converting阶段中GND wire和signal wire之间的阻抗是输入阻抗和输出阻抗，是较大的传导阻抗
Firstly, the capacitance between the GND wire and signal wire in the coupling stage is parasitic, which usually has a large capacitive reactance. But the impedance between the GND wire and signal wire in the converting stage is the input impedance and output impedance, which is the smaller conduction impedance.
% coupling阶段中的线上阻抗是线的阻抗，而converting阶段中的线上阻抗是器件的阻抗（等效阻抗）
Secondly, the impedance on the transmission lines in the coupling stage means the inherent impedance of the wire, which usually has a small resistance value. Meanwhile, the impedance on the transmission lines in the converting stage represents the impedance of electronic components (equivalent impedance), which usually has a larger resistance value.
\subsection{\textsc{Coupling Model}}\label{sec: appendix_coupling}
 To simplify the circuit, we convert the parasitic capacitance into impedance and conduct a delta-y transformation~\cite{laughton2013electrical} as shown in~\fig{fig: principle_coupling2}. There are three closed current loops in~\fig{fig: principle_coupling2}, where $I_a$ is the current flows in the signal line of the attack source, $I_g$ and $I_g$ are respectively defined as the propagating currents along the GND line and the signal line of the victim device. Applying Kirchhoff's voltage law (KVL) to these three current loops, we have 
In the coupling stage, the detail of impedance correspondence caused by delta-y transformation is shown as follows,
% \begin{equation}
%     \begin{aligned}
%         Z_{11} &= \frac{Z_{ga1}Z_{gs1}}{Z_{gs1}+Z_{ga1}+Z_{sa1}}\\[1pt]
%         Z_{12} &= \frac{Z_{sa1}Z_{gs1}}{Z_{gs1}+Z_{ga1}+Z_{sa1}}\\[1pt]
%         Z_{13} &= \frac{Z_{ga1}Z_{sa1}}{Z_{gs1}+Z_{ga1}+Z_{sa1}}\\[1pt]
%         Z_{21} &= \frac{Z_{ga2}Z_{gs2}}{Z_{gs2}+Z_{ga2}+Z_{vs2}}\\[1pt]
%         Z_{22} &= \frac{Z_{vs2}Z_{gs2}}{Z_{gs2}+Z_{ga2}+Z_{vs2}}\\[1pt]
%         Z_{23} &= \frac{Z_{ga2}Z_{vs2}}{Z_{gs2}+Z_{ga2}+Z_{vs2}}
%     \end{aligned} \label{con: appendix_coupling_yTransfer}
% \end{equation}
\begin{equation}
    \begin{aligned}
Z_{11}=\frac{Z_{g a 1} Z_{g s 1}}{Z_{g s 1}+Z_{g a 1}+Z_{s a 1}} & \ \ \ Z_{21}=\frac{Z_{g a 2} Z_{g s 2}}{Z_{g s 2}+Z_{g a 2}+Z_{v s 2}} \\
Z_{12}=\frac{Z_{s a 1} Z_{g s 1}}{Z_{g s 1}+Z_{g a 1}+Z_{s a 1}} & \ \ \ Z_{22}=\frac{Z_{v s 2} Z_{g s 2}}{Z_{g s 2}+Z_{g a 2}+Z_{v s 2}} \\
Z_{13}=\frac{Z_{g a 1} Z_{s a 1}}{Z_{g s 1}+Z_{g a 1}+Z_{s a 1}} & \ \ \ Z_{23}=\frac{Z_{g a 2} Z_{v s 2}}{Z_{g s 2}+Z_{g a 2}+Z_{v s 2}}
\end{aligned} \label{con: appendix_coupling_yTransfer}
\nonumber
\end{equation}
Applying Kirchhoff's voltage law (KVL) to these three current loops, we have 
\vspace{-8pt}
\begin{equation}
    \begin{aligned}
        Z_{11}(I_a-I_g)+Z_{13}(I_a-I_g-I_s)-V_s=0\\[1pt]
        Z_{11}(I_a-I_g)+(Z_{12}+Z{v}+Z_{22})I_s-Z_{21}I_g-Z_gI_g=0\\[1pt]
        (Z_{12}+Z{v}+Z_{22})I_s+Z_{23}(I_s+I_g)-Z_{13}(I_a-I_g-I_v)=0\label{con: appendix_cp}
    \end{aligned}
    \nonumber
\end{equation}
We define the CM current caused by the attack signal as the average current that flows on both the GND line and the signal line of the victim device,
% \begin{gather}
% % \setlength{\abovedisplayskip}{1pt}
% % \setlength{\belowdisplayskip}{1pt}
%     I_{CM}=\frac{I_g+I_s}{2}=\mu V_s\label{eq: appendix_ICM_Vs}
% \end{gather}
\begin{equation}
    \begin{aligned}
    I_{CM}=\frac{I_g+I_s}{2}=\mu V_s\label{eq: appendix_ICM_Vs}
    \end{aligned}
\end{equation}
where the coefficient $\mu$ represents the coupling factor, which can be expressed as:
\begin{equation}
\begin{aligned}
   \mu = \frac{(Z_{11}+Z_{13})(Z_{12}+Z_{22}+Z_{v})+Z_{13}(Z_{21}+Z_{g}+Z_{11})}{F}\\
    F =Z_{11}Z_{12}Z_{21}+Z_{11}Z_{13}Z_{21}+Z_{11}Z_{12}Z_{23}+Z_{12}Z_{13}Z_{21}+\\Z_{11}Z_{13}Z_{23}+Z_{12}Z_{13}Z_{23}+Z_{11}Z_{21}Z_{22}+Z_{11}Z_{21}Z_{23}+\\Z_{11}Z_{22}Z_{23}+Z_{13}Z_{21}Z_{22}+Z_{13}Z_{21}Z_{23}+Z_{13}Z_{22}Z_{23}+\\Z_{11}Z_{12}Z_{g}+Z_{11}Z_{13}Z_{g}+Z_{12}Z_{13}Z_{g}+Z_{11}Z_{22}Z_{g}+\\Z_{11}Z_{23}Z_{g}+Z_{13}Z_{22}Z_{g}+Z_{13}Z_{23}Z_{g}+Z_{11}Z_{21}Z_{v}+\\Z_{11}Z_{23}Z_{v}+Z_{13}Z_{21}Z_{v}+Z_{13}Z_{23}Z_{v}+Z_{11}Z_{g}Z_{v}+Z_{13}Z_{g}Z_{v}
    \label{con: appendix_mu}
    \nonumber
\end{aligned}
\end{equation}

At last, the expression of the matrix $x_{cp}$ and $b_{cp}$ are listed as follows,
\vspace{-3pt}
\begin{equation}
    \begin{aligned}
        x_{cp} &=\begin{bmatrix}
         I_a &  I_g & I_s 
        \end{bmatrix}
        ^T\\
        b_{cp} &= \begin{bmatrix}
         V_s & 0 & 0 
        \end{bmatrix}
        ^T \label{con: appendix_xcp_bcp}
    \end{aligned}
\end{equation}

% \begin{equation}
%     \mu = \frac{(Z_{11}+Z_{13})(Z_{12}+Z_{22}+Z_{v})+Z_{13}(Z_{21}+Z_{g}+Z_{11})}{\splitfrac{Z_{11}Z_{12}Z_{21}+Z_{11}Z_{13}Z_{21}+Z_{11}Z_{12}Z_{23}+Z_{12}Z_{13}Z_{21}}{\splitfrac{+Z_{11}Z_{13}Z_{23}+Z_{12}Z_{13}Z_{23}+Z_{11}Z_{21}Z_{22}+Z_{11}Z_{21}Z_{23}}{\splitfrac{+Z_{11}Z_{22}Z_{23}+Z_{13}Z_{21}Z_{22}+Z_{13}Z_{21}Z_{23}+Z_{13}Z_{22}Z_{23}}{\splitfrac{+Z_{11}Z_{12}Z_{g}+Z_{11}Z_{13}Z_{g}+Z_{12}Z_{13}Z_{g}+Z_{11}Z_{22}Z_{g}}{\splitfrac{+Z_{11}Z_{23}Z_{g}+Z_{13}Z_{22}Z_{g}+Z_{13}Z_{23}Z_{g}}{\splitfrac{+Z_{11}Z_{21}Z_{v}+Z_{11}Z_{23}Z_{v}+Z_{13}Z_{21}Z_{v}}{+Z_{13}Z_{23}Z_{v}+Z_{11}Z_{g}Z_{v}+Z_{13}Z_{g}Z_{v}}}}}}}}\label{con: mu}
% \end{equation}

\subsection{\textsc{Conversion Model}}\label{sec: appendix_conversion}
In the converting stage, the detail of impedance correspondence caused by delta-y transformation is shown as follows,
\vspace{-3pt}
% \begin{equation}
%     \begin{aligned}
%         Z_1 &= Z_{3I}\\[1pt]
%         Z_2 &= \frac{Z_LZ_{1I}}{Z_L+Z_{1I}+Z_{1O}}\\[1pt]
%         Z_3 &= \frac{Z_RZ_{2I}}{Z_R+Z_{2I}+Z_{2O}}\\[1pt]
%         Z_4 &= \frac{Z_{1I}Z_{1O}}{Z_L+Z_{1I}+Z_{1O}}\\[1pt]
%         Z_5 &= \frac{Z_{2I}Z_{2O}}{Z_R+Z_{2I}+Z_{2O}}\\[1pt]
%         Z_6 &= \frac{Z_LZ_{1O}}{Z_L+Z_{1I}+Z_{1O}}\\[1pt]
%         Z_7 &= \frac{Z_RZ_{2O}}{Z_R+Z_{2I}+Z_{2O}}\\[1pt]
%         Z_8 &= Z_{3O} \label{con: appendix_conversion_yTransfer}
%     \end{aligned}
% \end{equation}
\begin{equation}
    \begin{aligned}
Z_{1}=Z_{3 I} &\ \ Z_{5}=\frac{Z_{2 I} Z_{2 O}}{Z_{R}+Z_{2 I}+Z_{2 O}} \\
Z_{2}=\frac{Z_{L} Z_{1 I}}{Z_{L}+Z_{1 I}+Z_{1 O}} &\ \ Z_{6}=\frac{Z_{L} Z_{1 O}}{Z_{L}+Z_{1 I}+Z_{1 O}} \\
Z_{3}=\frac{Z_{R} Z_{2 I}}{Z_{R}+Z_{2 I}+Z_{2 O}} &\ \ Z_{7}=\frac{Z_{R} Z_{2 O}}{Z_{R}+Z_{2 I}+Z_{2 O}} \\
Z_{4}=\frac{Z_{1 I} Z_{1 O}}{Z_{L}+Z_{1 I}+Z_{1 O}} &\ \ Z_{8}=Z_{3 O}
\end{aligned}
% \nonumber
\end{equation}
We define the input DM voltage $V_{DM, I}$ as the voltage difference between two transmission lines on the input side, i.e., $V_{DM, I} = V_1-V_2$, and the input CM current $I_{CM}$ as the total current that flows on both transmission lines, i.e., $I_{CM} = I_1+I_2-I_3-I_4$. Besides, according to Kirchhoff laws~\cite{laughton2013electrical}, we have
% \begin{equation}
%     \begin{aligned}
%         % \small
%         % \setlength{\abovedisplayskip}{1pt}
%         % \setlength{\belowdisplayskip}{1pt}
%         I_1 - \frac{V_1-V_3}{Z_2} - \frac{V_1-V_2}{Z_1} &= 0 \\[1pt]
%         I_2 + \frac{V_1-V_2}{Z_1} + \frac{V_4-V_2}{Z_3} &= 0 \\[1pt]
%         \frac{V_1-V_3}{Z_2} - \frac{V_3-V_5}{Z_6}- \frac{V_3}{Z_4} &= 0\\[1pt]
%         \frac{V_6-V_4}{Z_7} - \frac{V_4-V_2}{Z_3} - \frac{V_4}{Z_5} &= 0\\[1pt]
%         \frac{V_3-V_5}{Z_6} - \frac{V_5-V_6}{Z_8} &= I_3\\[1pt]
%         \frac{V_5-V_6}{Z_8} - \frac{V_6-V_4}{Z_7} &= I_4 
%     \label{con}
%     \end{aligned}
% \end{equation}
% \begin{equation}
% \begin{array}{cc}
% I_{1}-\frac{V_{1}-V_{3}}{Z_{2}}-\frac{V_{1}-V_{2}}{Z_{1}}=0 & \frac{V_{6}-V_{4}}{Z_{7}}-\frac{V_{4}-V_{2}}{Z_{3}}-\frac{V_{4}}{Z_{5}}=0 \\
% I_{2}+\frac{V_{1}-V_{2}}{Z_{1}}+\frac{V_{4}-V_{2}}{Z_{3}}=0 & \frac{V_{3}-V_{5}}{Z_{6}}-\frac{V_{5}-V_{6}}{Z_{8}}=I_{3} \\
% \frac{V_{1}-V_{3}}{Z_{2}}-\frac{V_{3}-V_{5}}{Z_{6}}-\frac{V_{3}}{Z_{4}}=0 & \frac{V_{5}-V_{6}}{Z_{8}}-\frac{V_{6}-V_{4}}{Z_{7}}=I_{4}
% \end{array}
% \end{equation}
\begin{equation}
\begin{aligned}
I_{1}-\frac{V_{1}-V_{3}}{Z_{2}}-\frac{V_{1}-V_{2}}{Z_{1}}=0 &\ \ \  \frac{V_{6}-V_{4}}{Z_{7}}-\frac{V_{4}-V_{2}}{Z_{3}}=\frac{V_{4}}{Z_{5}} \\
I_{2}+\frac{V_{1}-V_{2}}{Z_{1}}+\frac{V_{4}-V_{2}}{Z_{3}}=0 &\ \ \  \frac{V_{3}-V_{5}}{Z_{6}}-\frac{V_{5}-V_{6}}{Z_{8}}=I_{3} \\
\frac{V_{1}-V_{3}}{Z_{2}}-\frac{V_{3}-V_{5}}{Z_{6}}-\frac{V_{3}}{Z_{4}}=0 &\ \ \  \frac{V_{5}-V_{6}}{Z_{8}}-\frac{V_{6}-V_{4}}{Z_{7}}=I_{4}
\end{aligned}
\nonumber
\end{equation}
Assume the output voltage $ V_{DM, O} = V_5- V_6$ as the output of the victim's device, i.e., the voltage difference across $Z_8$. By combining above equations yields the results for $ V_{DM, O}$,
\begin{gather}
\setlength{\abovedisplayskip}{1pt}
\setlength{\belowdisplayskip}{1pt}
    V_{DM,O} = k_1 V_{DM,I}+k_2 I_{CM}+k_3 I_3+k_4 I_4\label{con: V_DM_O}
\end{gather}
where $k_1$, $k_2$, $k_3$ and $k_4$ are constant coefficients formed by the impedance:
\vspace{-2pt}
\begin{equation}
\begin{aligned}
     k_1 &= \frac{Z_8(Z_4+Z_5)}{
     \splitfrac{(Z_6+Z_7+Z_8)(Z_2+Z_3+Z_4+Z_5)}{+(Z_2+Z_3)(Z_4+Z_5)}}\\
     k_2 &= \frac{Z_8(Z_3Z_4-Z_2Z_5)}{
     \splitfrac{(Z_6+Z_7+Z_8)(Z_2+Z_3+Z_4+Z_5)}{+(Z_2+Z_3)(Z_4+Z_5)}}\\
     k_3 &= -\frac{Z_8[Z_6(Z_2+Z_3+Z_4+Z_5)+Z_2(Z_4+Z_5)]}{
     \splitfrac{(Z_6+Z_7+Z_8)(Z_2+Z_3+Z_4+Z_5)}{+(Z_2+Z_3)(Z_4+Z_5)}} \label{con: appendix_k}
\end{aligned}
\end{equation}
\vspace{-2pt}
\begin{equation}
\begin{aligned}
     k_4 &= \frac{Z_8[Z_7(Z_2+Z_3+Z_4+Z_5)+Z_3(Z_4+Z_5)]}{
     \splitfrac{(Z_6+Z_7+Z_8)(Z_2+Z_3+Z_4+Z_5)}{+(Z_2+Z_3)(Z_4+Z_5)}}
\end{aligned}
\nonumber
\end{equation}
\vspace{-10pt}

\eq{con: define_vdmo} shows the output voltage $V_{DM, O}$ is combined with two parts: the input DM voltage $V_{DM, I}$, the input CM current $I_{CM}$, the output current $I_3$ and $I_4$. Therefore, the coefficient $k_2$ represents the CM-DM conversion degree, which can be decomposed as:
\vspace{-3pt}
\begin{equation}
\begin{aligned}
   k_2 &= c_1c_2(h_1+h_2)\ \ \ \ \ \ \ \ \ \ \ 
   h_1 = Z_R(Z_{1O}-Z_{2O})\\
   h_2 &= Z_{2O}(Z_L-Z_R)\\
   c_1 &= \frac{Z_8}{
    \splitfrac{(Z_6+Z_7+Z_8)(Z_2+Z_3+Z_4+Z_5)}{+(Z_2+Z_3)(Z_4+Z_5)}}\\[1pt]
   c_2 &= \frac{Z_{1I}Z_{2I}}{(Z_L+Z_{1I}+Z_{1O})(Z_R+Z_{2I}+Z_{2O})}
\end{aligned}
\end{equation}
% \begin{equation}
% \begin{aligned}
% k_2 = c_1c_2(h_1+h_2)\\
% h_1 = Z_R(Z_{1O}-Z_{2O}) &\ \ \  h_2 = Z_{2O}(Z_L-Z_R)
% \end{aligned}
% \end{equation}
where $c_1$ and $c_2$ are constants, $h_1$ and $h_2$ are respectively composed of parasitic impedance and line impedance of the circuit, which reflect the degree of asymmetry, so we name it asymmetric factor.

% \begin{gather}
% I_1-\frac{V_1-V_3}{Z_2}-\frac{V_1-V_2}{Z_1}=0\label{con:eq1}\\[5pt]
% I_2+\frac{V_1-V_2}{Z_1}+\frac{V_4-V_2}{Z_3}=0\\[5pt]
% \frac{V_1-V_3}{Z_2}-\frac{V_3-V_5}{Z_6}-\frac{V_3}{Z_4}=0\\[5pt]
% \frac{V_6-V_4}{Z_7}-\frac{V_4-V_2}{Z_3}-\frac{V_4}{Z_5}=0\\[5pt]
% \frac{V_3-V_5}{Z_6}-\frac{V_5-V_6}{Z_8}=I_3\\[5pt]
% \frac{V_5-V_6}{Z_8}-\frac{V_6-V_4}{Z_7}=I_4\\[5pt]
% I_1+I_2=I_{CM}+I_3+I_4\\[5pt]
% V_1-V_2=V_{DM,I}
% \end{gather}

% Coefficient $k_1$, $k_2$ and $k_3$, $k_4$ is shown as follows,
% \begin{gather}
%      k_1 = \frac{Z_8(Z_4+Z_5)}{
%      \splitfrac{(Z_6+Z_7+Z_8)(Z_2+Z_3+Z_4+Z_5)}{+(Z_2+Z_3)(Z_4+Z_5)}}\\[5pt]
%      k_2 = \frac{Z_8(Z_3Z_4-Z_2Z_5)}{
%      \splitfrac{(Z_6+Z_7+Z_8)(Z_2+Z_3+Z_4+Z_5)}{+(Z_2+Z_3)(Z_4+Z_5)}}\\[5pt]
%      k_3 = -\frac{Z_8[Z_6(Z_2+Z_3+Z_4+Z_5)+Z_2(Z_4+Z_5)]}{
%      \splitfrac{(Z_6+Z_7+Z_8)(Z_2+Z_3+Z_4+Z_5)}{+(Z_2+Z_3)(Z_4+Z_5)}}\\[5pt]
%      k_4 = \frac{Z_8[Z_7(Z_2+Z_3+Z_4+Z_5)+Z_3(Z_4+Z_5)]}{
%      \splitfrac{(Z_6+Z_7+Z_8)(Z_2+Z_3+Z_4+Z_5)}{+(Z_2+Z_3)(Z_4+Z_5)}}\\[5pt]
%      \label{con: k}
% \end{gather}

% \newpage
According to Kirchhoff laws~\cite{laughton2013electrical}, the relationships of impedance, voltages, and currents can be expressed in the form of $A_{cv}x_{cv}=b_{cv}$, where}
\begin{equation}
    \begin{aligned}
        A_{cv} &= \begin{bmatrix}
            A_{cv1} & A_{cv2}
            \end{bmatrix}\\
        x_{cv} &= \begin{bmatrix}
            V_1 &  V_2 & V_3 & V_4 & V_5 & V_6 & I_1 & I_2 
            \end{bmatrix}^T\\
        b_{cv} &= \begin{bmatrix}
            0 & 0 & 0 & 0 & I_3 & I_4 & I_{CM}+I_3+I_4 & V_{DM,I}
            \end{bmatrix}^T
    \end{aligned}
    \nonumber
\end{equation}
where
\begin{equation}
    A_{cv1}=\begin{bmatrix}
      -\frac{1}{Z_1}-\frac{1}{Z_2} & \frac{1}{Z_1} & \frac{1}{Z_2} \\
      \frac{1}{Z_1}& -\frac{1}{Z_1}-\frac{1}{Z_3} & 0\\
      \frac{1}{Z_2}& 0 & -\frac{1}{Z_2}-\frac{1}{Z_4}-\frac{1}{Z_6}\\
      0 & \frac{1}{Z_3} & 0 \\
      0 & 0 & \frac{1}{Z_6}\\
      0 & 0 & 0 \\
      0 & 0 & 0 \\
      1 & -1 & 0 \end{bmatrix}
      \nonumber
\end{equation}
\begin{equation}
    A_{cv2}=\begin{bmatrix}
        0 & 0 & 0 & 1 & 0\\
        \frac{1}{Z_3} & 0 & 0 & 0 & 1\\
        & \frac{1}{Z_6} & 0 & 0 & 0\\
        -\frac{1}{Z_3}-\frac{1}{Z_5}-\frac{1}{Z_7} & 0 & \frac{1}{Z_7} & 0 & 0\\
        0 & -\frac{1}{Z_6}-\frac{1}{Z_8} & \frac{1}{Z_8} & 0 & 0\\
        \frac{1}{Z_7} & \frac{1}{Z_8} & -\frac{1}{Z_7}-\frac{1}{Z_8} & 0 & 0\\
        0 & 0 & 0 & 1 & 1\\
        0 & 0 & 0 & 0 & 0
        \end{bmatrix}
        \nonumber
\end{equation}

% \begin{gather}
%     Z_1=Z_{3I}\\
%     Z_2=\frac{Z_LZ_{1I}}{Z_L+Z_{1I}+Z_{1O}}\\
%     Z_3=\frac{Z_RZ_{2I}}{Z_R+Z_{2I}+Z_{2O}}\\
%     Z_4=\frac{Z_{1I}Z_{1O}}{Z_L+Z_{1I}+Z_{1O}}\\
%     Z_5=\frac{Z_{2I}Z_{2O}}{Z_R+Z_{2I}+Z_{2O}}\\
%     Z_6=\frac{Z_LZ_{1O}}{Z_L+Z_{1I}+Z_{1O}}\\
%     Z_7=\frac{Z_RZ_{2O}}{Z_R+Z_{2I}+Z_{2O}}\\
%     Z_8=Z_{3O}
% \end{gather}

% \begin{equation}
%   \begin{aligned}
%    V_{DM,O} &= V_5-V_6=x[5]-x[6] \\
%    &=k_1[(Z_4+Z_5)V_{DM,I}+(Z_3Z_4-Z_2Z_5)I_{CM}]
%   \end{aligned}
% \end{equation}

% Coefficient $k_1$, $k_2$ and $c_1$, $c_2$ is shown as follows,
% \begin{gather}
%      k_1 = \frac{Z_8(Z_4+Z_5)}{(Z_6+Z_7+Z_8)(Z_2+Z_3+Z_4+Z_5)+(Z_2+Z_3)(Z_4+Z_5)}\\
%      k_2 = \frac{Z_8(Z_3Z_4-Z_2Z_5)}{(Z_6+Z_7+Z_8)(Z_2+Z_3+Z_4+Z_5)+(Z_2+Z_3)(Z_4+Z_5)}\\
%     c_1 = \frac{Z_8}{(Z_6+Z_7+Z_8)(Z_2+Z_3+Z_4+Z_5)+(Z_2+Z_3)(Z_4+Z_5)}\\
%     c_2 = \frac{Z_{1I}Z_{2I}}{(Z_L+Z_{1I}+Z_{1O})(Z_R+Z_{2I}+Z_{2O})}
% \end{gather}

% \begin{gather}
%      k_1 = \frac{Z_8(Z_4+Z_5)}{
%      \splitfrac{(Z_6+Z_7+Z_8)(Z_2+Z_3+Z_4+Z_5)}{+(Z_2+Z_3)(Z_4+Z_5)}}\\
%      k_2 = \frac{Z_8(Z_3Z_4-Z_2Z_5)}{
%      \splitfrac{(Z_6+Z_7+Z_8)(Z_2+Z_3+Z_4+Z_5)}{+(Z_2+Z_3)(Z_4+Z_5)}}\\
%     c_1 = \frac{Z_8}{
%     \splitfrac{(Z_6+Z_7+Z_8)(Z_2+Z_3+Z_4+Z_5)}{+(Z_2+Z_3)(Z_4+Z_5)}}\\
%     c_2 = \frac{Z_{1I}Z_{2I}}{(Z_L+Z_{1I}+Z_{1O})(Z_R+Z_{2I}+Z_{2O})}
% \end{gather}

\subsection{\textsc{Modeling Simulation}}\label{sec: appendix_modeling_simulation}
% We also use Matlab to simulate our coupling and conversion models and define parameters as follows.
\blue{The simulation parameters of the coupling model and conversion model are defined as follows.}

\textit{(1) Simulation Parameters in Coupling Stage.}
\begin{equation}
    \begin{aligned}
    V_s &= 300 Vpp \\[1pt]
    Z_{ga1} &= 1000000+\frac{1}{j\times 1\times 10^{-5} \omega } \Omega \\[1pt]
    Z_{sa1} &= 1000000+\frac{1}{j\times 0.99\times 10^{-5} \omega }\Omega \\[1pt]
    Z_{ga2} &= 1000000+\frac{1}{j\times 1.01\times 10^{-5} \omega }\Omega \\[1pt]
    Z_{sa2} &= 1000000+\frac{1}{j\times 0.98\times 10^{-5} \omega }\Omega \\[1pt]
    Z_{gs1} &= 1000000+\frac{1}{j\times 1.21\times 10^{-5} \omega }\Omega \\[1pt]
    Z_{gs1} &= 1000000+\frac{1}{j\times 1.19\times 10^{-5} \omega }\Omega \\[1pt]
    Z_{s} &= 0.00099+j\times 5\times 10^{-6} \omega+\frac{1}{j\times 1.1\times 10^{-9} \omega }\Omega \\[1pt]
    Z_{g} &= 0.0001001+j\times 4.43\times 10^{-6} \omega+\frac{1}{j\times 0.99\times 10^{-9} \omega }\Omega
    \end{aligned}\label{eq: simulation_coupling}
    \nonumber
\end{equation}
\textit{(2) Simulation Parameters in Converting Stage.}
\begin{equation}
    \begin{aligned}
    Z_{1I} &= 1000000+\frac{1}{j\times 1\times 10^{-7} \omega }\Omega \\[1pt]
    Z_{2I} &= 1000000+\frac{1}{j\times 1.1\times 10^{-7} \omega }\Omega \\[1pt]
    Z_{1O} &= 1000000+\frac{1}{j\times 0.99\times 10^{-7} \omega }\Omega \\[1pt]
    Z_{2O} &= 1000000+\frac{1}{j\times 1.01\times 10^{-7} \omega }\Omega \\[1pt]
    Z_{3I} &= 1000000+\frac{1}{j\times 1.21\times 10^{-6} \omega }\Omega \\[1pt]
    Z_{3O} &= 1000000+\frac{1}{j\times 1.19\times 10^{-6} \omega }\Omega \\[1pt]
    Z_{R} &= 19.99+j\times 0.05 \omega+\frac{1}{j\times 1.1\times 10^{-3} \omega }\Omega \\[1pt]
    Z_{L} &= 20.01+j\times 0.049 \omega+\frac{1}{j\times 1.2\times 10^{-3} \omega }\Omega
    \end{aligned}
    \nonumber
\end{equation}

% ===========complete formulation of A_cv
% \newpage
% \begin{equation}
% A_{cv}=\begin{bmatrix}
%   -\frac{1}{Z_1}-\frac{1}{Z_2} & \frac{1}{Z_1} & \frac{1}{Z_2} & 0 & 0 & 0 & 1 & 0\\
%   \frac{1}{Z_1}& -\frac{1}{Z_1}-\frac{1}{Z_3} & 0 & \frac{1}{Z_3} & 0 & 0 & 0 & 1\\
%   \frac{1}{Z_2}& 0 & -\frac{1}{Z_2}-\frac{1}{Z_4}-\frac{1}{Z_6} & 0 & \frac{1}{Z_6} & 0 & 0 & 0\\
%   0 & \frac{1}{Z_3} & 0 & -\frac{1}{Z_3}-\frac{1}{Z_5}-\frac{1}{Z_7} & 0 & \frac{1}{Z_7} & 0 & 0\\
%   0 & 0 & \frac{1}{Z_6} & 0 & -\frac{1}{Z_6}-\frac{1}{Z_8} & \frac{1}{Z_8} & 0 & 0\\
%   0 & 0 & 0 & \frac{1}{Z_7} & \frac{1}{Z_8} & -\frac{1}{Z_7}-\frac{1}{Z_8} & 0 & 0\\
%   0 & 0 & 0 & 0 & 0 & 0 & 1 & 1\\
%   1 & -1 & 0 & 0 & 0 & 0 & 0 & 0
%   \end{bmatrix}
% \end{equation}
